# Supplementary material for: Measurements of the electric and magnetic form factors of the neutron for time-like momentum transfer
Source: arXiv:2212.07071 source file (2023-03-29)
Supplement: Supplementary file 2 [file supplenmentary.pdf]

# Supplemental Material for “Measurements of the electric and magnetic form factors of the neutron for time-like momentum transfer

M. Ablikim<sup>1</sup>, M. N. Achasov<sup>13,b</sup>, P. Adlarson<sup>73</sup>, R. Aliberti<sup>34</sup>, A. Amoroso<sup>72A,72C</sup>, M. R. An<sup>38</sup>, Q. An<sup>69,56</sup>, Y. Bai<sup>55</sup>, O. Bakina<sup>35</sup>, I. Balossino<sup>29A</sup>, Y. Ban<sup>45,g</sup>, V. Batozskaya<sup>1,43</sup>, K. Begzsuren<sup>31</sup>, N. Berger<sup>34</sup>, M. Bertani<sup>28A</sup>, D. Bettoni<sup>29A</sup>, F. Bianchi<sup>72A,72C</sup>, E. Bianco<sup>72A,72C</sup>, J. Bloms<sup>66</sup>, A. Bortone<sup>72A,72C</sup>, I. Boyko<sup>35</sup>, R. A. Briere<sup>5</sup>, A. Brueggemann<sup>66</sup>, H. Cai<sup>74</sup>, X. Cai<sup>1,56</sup>, A. Calcaterra<sup>28A</sup>, G. F. Cao<sup>1,61</sup>, N. Cao<sup>1,61</sup>, S. A. Cetin<sup>60A</sup>, J. F. Chang<sup>1,56</sup>, T. T. Chang<sup>75</sup>, W. L. Chang<sup>1,61</sup>, G. R. Che<sup>42</sup>, G. Chelkov<sup>35,a</sup>, C. Chen<sup>42</sup>, Chao Chen<sup>53</sup>, G. Chen<sup>1</sup>, H. S. Chen<sup>1,61</sup>, M. L. Chen<sup>1,56,61</sup>, S. J. Chen<sup>41</sup>, S. M. Chen<sup>59</sup>, T. Chen<sup>1,61</sup>, X. R. Chen<sup>30,61</sup>, X. T. Chen<sup>1,61</sup>, Y. B. Chen<sup>1,56</sup>, Y. Q. Chen<sup>33</sup>, Z. J. Chen<sup>25,h</sup>, W. S. Cheng<sup>72C</sup>, S. K. Choi<sup>10A</sup>, X. Chu<sup>42</sup>, G. Cibinetto<sup>29A</sup>, S. C. Coen<sup>4</sup>, F. Cossio<sup>72C</sup>, J. J. Cui<sup>48</sup>, H. L. Dai<sup>1,56</sup>, J. P. Dai<sup>77</sup>, A. Dbeysy<sup>19</sup>, R. E. de Boer<sup>4</sup>, D. Dedovich<sup>35</sup>, Z. Y. Deng<sup>1</sup>, A. Denig<sup>34</sup>, I. Denysenko<sup>35</sup>, M. Destefanis<sup>72A,72C</sup>, F. De Mori<sup>72A,72C</sup>, B. Ding<sup>64,1</sup>, Y. Ding<sup>33</sup>, Y. Ding<sup>39</sup>, J. Dong<sup>1,56</sup>, L. Y. Dong<sup>1,61</sup>, M. Y. Dong<sup>1,56,61</sup>, X. Dong<sup>74</sup>, S. X. Du<sup>79</sup>, Z. H. Duan<sup>41</sup>, P. Egorov<sup>35,a</sup>, Y. L. Fan<sup>74</sup>, J. Fang<sup>1,56</sup>, S. S. Fang<sup>1,61</sup>, W. X. Fang<sup>1</sup>, Y. Fang<sup>1</sup>, R. Farinelli<sup>29A</sup>, L. Fava<sup>72B,72C</sup>, F. Feldbauer<sup>4</sup>, G. Felici<sup>28A</sup>, C. Q. Feng<sup>69,56</sup>, J. H. Feng<sup>57</sup>, K. Fischer<sup>67</sup>, M. Fritsch<sup>4</sup>, C. Fritzsche<sup>66</sup>, C. D. Fu<sup>1</sup>, Y. W. Fu<sup>1</sup>, H. Gao<sup>61</sup>, Y. N. Gao<sup>45,g</sup>, Yang Gao<sup>69,56</sup>, S. Garbolino<sup>72C</sup>, I. Garzia<sup>29A,29B</sup>, P. T. Ge<sup>74</sup>, Z. W. Ge<sup>41</sup>, C. Geng<sup>57</sup>, E. M. Gersabeck<sup>65</sup>, A. Gilman<sup>67</sup>, K. Goetzen<sup>14</sup>, L. Gong<sup>39</sup>, W. X. Gong<sup>1,56</sup>, W. Gradl<sup>34</sup>, S. Gramigna<sup>29A,29B</sup>, M. Greco<sup>72A,72C</sup>, M. H. Gu<sup>1,56</sup>, Y. T. Gu<sup>16</sup>, C. Y. Guan<sup>1,61</sup>, Z. L. Guan<sup>22</sup>, A. Q. Guo<sup>30,61</sup>, L. B. Guo<sup>40</sup>, R. P. Guo<sup>47</sup>, Y. P. Guo<sup>12,f</sup>, A. Guskov<sup>35,a</sup>, X. T. H.<sup>1,61</sup>, W. Y. Han<sup>38</sup>, X. Q. Hao<sup>20</sup>, F. A. Harris<sup>63</sup>, K. K. He<sup>53</sup>, K. L. He<sup>1,61</sup>, F. H. Heinsius<sup>4</sup>, C. H. Heinz<sup>34</sup>, Y. K. Heng<sup>1,56,61</sup>, C. Herold<sup>58</sup>, T. Holtmann<sup>4</sup>, P. C. Hong<sup>12,f</sup>, G. Y. Hou<sup>1,61</sup>, Y. R. Hou<sup>61</sup>, Z. L. Hou<sup>1</sup>, H. M. Hu<sup>1,61</sup>, J. F. Hu<sup>54,i</sup>, T. Hu<sup>1,56,61</sup>, Y. Hu<sup>1</sup>, G. S. Huang<sup>69,56</sup>, K. X. Huang<sup>57</sup>, L. Q. Huang<sup>30,61</sup>, X. T. Huang<sup>48</sup>, Y. P. Huang<sup>1</sup>, T. Hussain<sup>71</sup>, N. Hüsken<sup>27,34</sup>, W. Imoehl<sup>27</sup>, M. Irshad<sup>69,56</sup>, J. Jackson<sup>27</sup>, S. Jaeger<sup>4</sup>, S. Janchiv<sup>31</sup>, J. H. Jeong<sup>10A</sup>, Q. Ji<sup>1</sup>, Q. P. Ji<sup>20</sup>, X. B. Ji<sup>1,61</sup>, X. L. Ji<sup>1,56</sup>, Y. Y. Ji<sup>48</sup>, Z. K. Jia<sup>69,56</sup>, P. C. Jiang<sup>45,g</sup>, S. S. Jiang<sup>38</sup>, T. J. Jiang<sup>17</sup>, X. S. Jiang<sup>1,56,61</sup>, Y. Jiang<sup>61</sup>, J. B. Jiao<sup>48</sup>, Z. Jiao<sup>23</sup>, S. Jin<sup>41</sup>, Y. Jin<sup>64</sup>, M. Q. Jing<sup>1,61</sup>, T. Johansson<sup>73</sup>, X. K.<sup>1</sup>, S. Kabana<sup>32</sup>, N. Kalantar-Nayestanaki<sup>62</sup>, X. L. Kang<sup>9</sup>, X. S. Kang<sup>39</sup>, R. Kappert<sup>62</sup>, M. Kavatsyuk<sup>62</sup>, B. C. Ke<sup>79</sup>, A. Khoukaz<sup>66</sup>, R. Kiuchi<sup>1</sup>, R. Kliemt<sup>14</sup>, L. Koch<sup>36</sup>, O. B. Kolcu<sup>60A</sup>, B. Kopf<sup>4</sup>, M. Kuessner<sup>4</sup>, A. Kupsc<sup>43,73</sup>, W. Kühn<sup>36</sup>, J. J. Lane<sup>65</sup>, J. S. Lange<sup>36</sup>, P. Larin<sup>19</sup>, A. Lavania<sup>26</sup>, L. Lavezzi<sup>72A,72C</sup>, T. T. Lei<sup>69,k</sup>, Z. H. Lei<sup>69,56</sup>, H. Leithoff<sup>34</sup>, M. Lellmann<sup>34</sup>, T. Lenz<sup>34</sup>, C. Li<sup>46</sup>, C. Li<sup>42</sup>, C. H. Li<sup>38</sup>, Cheng Li<sup>69,56</sup>, D. M. Li<sup>79</sup>, F. Li<sup>1,56</sup>, G. Li<sup>1</sup>, H. Li<sup>69,56</sup>, H. B. Li<sup>1,61</sup>, H. J. Li<sup>20</sup>, H. N. Li<sup>54,i</sup>, Hui Li<sup>42</sup>, J. R. Li<sup>59</sup>, J. S. Li<sup>57</sup>, J. W. Li<sup>48</sup>, Ke Li<sup>1</sup>, L. J. Li<sup>1,61</sup>, L. K. Li<sup>1</sup>, Lei Li<sup>3</sup>, M. H. Li<sup>42</sup>, P. R. Li<sup>37,j,k</sup>, S. X. Li<sup>12</sup>, T. Li<sup>48</sup>, W. D. Li<sup>1,61</sup>, W. G. Li<sup>1</sup>, X. H. Li<sup>69,56</sup>, X. L. Li<sup>48</sup>, Xiaoyu Li<sup>1,61</sup>, Y. G. Li<sup>45,g</sup>, Z. J. Li<sup>57</sup>, Z. X. Li<sup>16</sup>, Z. Y. Li<sup>57</sup>, C. Liang<sup>41</sup>, H. Liang<sup>33</sup>, H. Liang<sup>1,61</sup>, H. Liang<sup>69,56</sup>, Y. F. Liang<sup>52</sup>, Y. T. Liang<sup>30,61</sup>, G. R. Liao<sup>15</sup>, L. Z. Liao<sup>48</sup>, J. Libby<sup>26</sup>, A. Limphirat<sup>58</sup>, D. X. Lin<sup>30,61</sup>, T. Lin<sup>1</sup>, B. X. Liu<sup>74</sup>, B. J. Liu<sup>1</sup>, C. Liu<sup>33</sup>, C. X. Liu<sup>1</sup>, D. Liu<sup>19,69</sup>, F. H. Liu<sup>51</sup>, Fang Liu<sup>1</sup>, Feng Liu<sup>6</sup>, G. M. Liu<sup>54,i</sup>, H. Li<sup>37,j,k</sup>, H. B. Liu<sup>16</sup>, H. M. Liu<sup>1,61</sup>, Huanhuan Liu<sup>1</sup>, Huihui Liu<sup>21</sup>, J. B. Liu<sup>69,56</sup>, J. L. Liu<sup>70</sup>, J. Y. Liu<sup>1,61</sup>, K. Liu<sup>1</sup>, K. Y. Liu<sup>39</sup>, Ke Liu<sup>22</sup>, L. Liu<sup>69,56</sup>, L. C. Liu<sup>42</sup>, Lu Liu<sup>42</sup>, M. H. Liu<sup>12,f</sup>, P. L. Liu<sup>1</sup>, Q. Liu<sup>61</sup>, S. B. Liu<sup>69,56</sup>, T. Liu<sup>12,f</sup>, W. K. Liu<sup>42</sup>, W. M. Liu<sup>69,56</sup>, X. Liu<sup>37,j,k</sup>, Y. Liu<sup>37,j,k</sup>, Y. B. Liu<sup>42</sup>, Z. A. Liu<sup>1,56,61</sup>, Z. Q. Liu<sup>48</sup>, X. C. Lou<sup>1,56,61</sup>, F. X. Lu<sup>57</sup>, H. J. Lu<sup>23</sup>, J. G. Lu<sup>1,56</sup>, X. L. Lu<sup>1</sup>, Y. Lu<sup>7</sup>, Y. P. Lu<sup>1,56</sup>, Z. H. Lu<sup>1,61</sup>, C. L. Luo<sup>40</sup>, M. X. Luo<sup>78</sup>, T. Luo<sup>12,f</sup>, X. L. Luo<sup>1,56</sup>, X. R. Lyu<sup>61</sup>, Y. F. Lyu<sup>42</sup>, F. C. Ma<sup>39</sup>, H. L. Ma<sup>1</sup>, J. L. Ma<sup>1,61</sup>, L. L. Ma<sup>48</sup>, M. M. Ma<sup>1,61</sup>, Q. M. Ma<sup>1</sup>, R. Q. Ma<sup>1,61</sup>, R. T. Ma<sup>61</sup>, X. Y. Ma<sup>1,56</sup>, Y. Ma<sup>45,g</sup>, F. E. Maas<sup>19</sup>, M. Maggiora<sup>72A,72C</sup>, S. Maldaner<sup>4</sup>, S. Malde<sup>67</sup>, A. Mangoni<sup>28B</sup>, Y. J. Mao<sup>45,g</sup>, Z. P. Mao<sup>1</sup>, S. Marcello<sup>72A,72C</sup>, Z. X. Meng<sup>64</sup>, J. G. Messchendorp<sup>14,62</sup>, G. Mezzadri<sup>29A</sup>, H. Miao<sup>1,61</sup>, T. J. Min<sup>41</sup>, R. E. Mitchell<sup>27</sup>, X. H. Mo<sup>1,56,61</sup>, N. Yu. Muchnoi<sup>13,b</sup>, Y. Nefedov<sup>35</sup>, F. Nerling<sup>19,d</sup>, I. B. Nikolaev<sup>13,b</sup>, Z. Ning<sup>1,56</sup>, S. Nisar<sup>11,l</sup>, Y. Niu<sup>48</sup>, S. L. Olsen<sup>61</sup>, Q. Ouyang<sup>1,56,61</sup>, S. Pacetti<sup>28B,28C</sup>, X. Pan<sup>53</sup>, Y. Pan<sup>55</sup>, A. Pathak<sup>33</sup>, Y. P. Pei<sup>69,56</sup>, M. Pelizaeus<sup>4</sup>, H. P. Peng<sup>69,56</sup>, K. Peters<sup>14,d</sup>, J. L. Ping<sup>40</sup>, R. G. Ping<sup>1,61</sup>, S. Plura<sup>34</sup>, S. Pogodin<sup>35</sup>, V. Prasad<sup>32</sup>, F. Z. Qi<sup>1</sup>, H. Qi<sup>69,56</sup>, H. R. Qi<sup>59</sup>, M. Qi<sup>41</sup>, T. Y. Qi<sup>12,f</sup>, S. Qian<sup>1,56</sup>, W. B. Qian<sup>61</sup>, C. F. Qiao<sup>61</sup>, J. J. Qin<sup>70</sup>, L. Q. Qin<sup>15</sup>, X. P. Qin<sup>12,f</sup>, X. S. Qin<sup>48</sup>, Z. H. Qin<sup>1,56</sup>, J. F. Qiu<sup>1</sup>, S. Q. Qu<sup>59</sup>, C. F. Redmer<sup>34</sup>, K. J. Ren<sup>38</sup>, A. Rivetti<sup>72C</sup>, V. Rodin<sup>62</sup>, M. Rolo<sup>72C</sup>, G. Rong<sup>1,61</sup>, Ch. Rosner<sup>19</sup>, S. N. Ruan<sup>42</sup>, A. Sarantsev<sup>35,c</sup>, Y. Schelhaas<sup>34</sup>, K. Schoenning<sup>73</sup>, M. Scodreggio<sup>29A,29B</sup>, K. Y. Shan<sup>12,f</sup>, W. Shan<sup>24</sup>, X. Y. Shan<sup>69,56</sup>, J. F. Shanguan<sup>53</sup>, L. G. Shao<sup>1,61</sup>, M. Shao<sup>69,56</sup>, C. P. Shen<sup>12,f</sup>, H. F. Shen<sup>1,61</sup>, W. H. Shen<sup>61</sup>, X. Y. Shen<sup>1,61</sup>, B. A. Shi<sup>61</sup>, H. C. Shi<sup>69,56</sup>, J. Y. Shi<sup>1</sup>, Q. Q. Shi<sup>53</sup>, R. S. Shi<sup>1,61</sup>, X. Shi<sup>1,56</sup>, J. J. Song<sup>20</sup>, T. Z. Song<sup>57</sup>, W. M. Song<sup>33,1</sup>, Y. X. Song<sup>45,g</sup>, S. Sosio<sup>72A,72C</sup>, S. Spataro<sup>72A,72C</sup>, F. Stieler<sup>34</sup>, Y. J. Su<sup>61</sup>, G. B. Sun<sup>74</sup>, G. X. Sun<sup>1</sup>, H. Sun<sup>61</sup>, H. K. Sun<sup>1</sup>, J. F. Sun<sup>20</sup>, K. Sun<sup>59</sup>, L. Sun<sup>74</sup>, S. S. Sun<sup>1,61</sup>, T. Sun<sup>1,61</sup>, W. Y. Sun<sup>33</sup>, Y. Sun<sup>9</sup>, Y. J. Sun<sup>69,56</sup>, Y. Z. Sun<sup>1</sup>, Z. T. Sun<sup>48</sup>, Y. X. Tan<sup>69,56</sup>, C. J. Tang<sup>52</sup>, G. Y. Tang<sup>1</sup>, J. Tang<sup>57</sup>, Y. A. Tang<sup>74</sup>, L. Y. Tao<sup>70</sup>, Q. T. Tao<sup>25,h</sup>, M. Tat<sup>67</sup>, J. X. Teng<sup>69,56</sup>, V. Thoren<sup>73</sup>, W. H. Tian<sup>50</sup>, W. H. Tian<sup>57</sup>, Y. Tian<sup>30,61</sup>, Z. F. Tian<sup>74</sup>, I. Uman<sup>60B</sup>, B. Wang<sup>1</sup>, B. L. Wang<sup>61</sup>, Bo Wang<sup>69,56</sup>, C. W. Wang<sup>41</sup>, D. Y. Wang<sup>45,g</sup>, F. Wang<sup>70</sup>, H. J. Wang<sup>37,j,k</sup>, H. P. Wang<sup>1,61</sup>, K. Wang<sup>1,56</sup>, L. L. Wang<sup>1</sup>, M. Wang<sup>48</sup>, Meng Wang<sup>1,61</sup>, S. Wang<sup>12,f</sup>, T. Wang<sup>12,f</sup>, T. J. Wang<sup>42</sup>, W. Wang<sup>57</sup>, W. Wang<sup>70</sup>, W. H. Wang<sup>74</sup>, W. P. Wang<sup>69,56</sup>, X. Wang<sup>45,g</sup>, X. F. Wang<sup>37,j,k</sup>, X. J. Wang<sup>38</sup>, X. L. Wang<sup>12,f</sup>, Y. Wang<sup>59</sup>, Y. D. Wang<sup>44</sup>, Y. F. Wang<sup>1,56,61</sup>, Y. H. Wang<sup>46</sup>, Y. N. Wang<sup>44</sup>, Y. Q. Wang<sup>1</sup>, Yaqian Wang<sup>18,1</sup>, Yi Wang<sup>59</sup>, Z. Wang<sup>1,56</sup>, Z. L. Wang<sup>70</sup>, Z. Y. Wang<sup>1,61</sup>, Ziyi Wang<sup>61</sup>, D. Wei<sup>68</sup>, D. H. Wei<sup>15</sup>, F. Weidner<sup>66</sup>, S. P. Wen<sup>1</sup>, C. W. Wenzel<sup>4</sup>, U. Wiedner<sup>4</sup>, G. Wilkinson<sup>67</sup>, M. Wolke<sup>73</sup>, L. Wollenberg<sup>4</sup>, C. Wu<sup>38</sup>, J. F. Wu<sup>1,61</sup>, L. H. Wu<sup>1</sup>, L. J. Wu<sup>1,61</sup>, X. Wu<sup>12,f</sup>, X. H. Wu<sup>33</sup>, Y. Wu<sup>69</sup>, Y. J. Wu<sup>30</sup>, Z. Wu<sup>1,56</sup>, L. Xia<sup>69,56</sup>, X. M. Xian<sup>38</sup>, T. Xiang<sup>45,g</sup>, D. Xiao<sup>37,j,k</sup>, G. Y. Xiao<sup>41</sup>, H. Xiao<sup>12,f</sup>, S. Y. Xiao<sup>1</sup>, Y. L. Xiao<sup>12,f</sup>, Z. J. Xiao<sup>40</sup>, C. Xie<sup>41</sup>, X. H. Xie<sup>45,g</sup>, Y. Xie<sup>48</sup>, Y. G. Xie<sup>1,56</sup>, Y. H. Xie<sup>6</sup>, Z. P. Xie<sup>69,56</sup>, T. Y. Xing<sup>1,61</sup>, C. F. Xu<sup>1,61</sup>, C. J. Xu<sup>57</sup>, G. F. Xu<sup>1</sup>, H. Y. Xu<sup>64</sup>, Q. J. Xu<sup>17</sup>, W. L. Xu<sup>64</sup>, X. P. Xu<sup>53</sup>, Y. C. Xu<sup>76</sup>, Z. P. Xu<sup>41</sup>, F. Yan<sup>12,f</sup>, L. Yan<sup>12,f</sup>, W. B. Yan<sup>69,56</sup>, W. C. Yan<sup>79</sup>, X. Q. Yan<sup>1</sup>, H. J. Yang<sup>49,e</sup>, H. L. Yang<sup>33</sup>, H. X. Yang<sup>1</sup>, Tao Yang<sup>1</sup>, Y. Yang<sup>12,f</sup>, Y. F. Yang<sup>42</sup>, Y. X. Yang<sup>1,61</sup>, Yifan Yang<sup>1,61</sup>, M. Ye<sup>1,56</sup>,

M. H. Ye<sup>8</sup>, J. H. Yin<sup>1</sup>, Z. Y. You<sup>57</sup>, B. X. Yu<sup>1,56,61</sup>, C. X. Yu<sup>42</sup>, G. Yu<sup>1,61</sup>, T. Yu<sup>70</sup>, X. D. Yu<sup>45,g</sup>, C. Z. Yuan<sup>1,61</sup>, L. Yuan<sup>2</sup>, S. C. Yuan<sup>1</sup>, X. Q. Yuan<sup>1</sup>, Y. Yuan<sup>1,61</sup>, Z. Y. Yuan<sup>57</sup>, C. X. Yue<sup>38</sup>, A. A. Zafar<sup>71</sup>, F. R. Zeng<sup>48</sup>, X. Zeng<sup>12,f</sup>, Y. Zeng<sup>25,h</sup>, Y. J. Zeng<sup>1,61</sup>, X. Y. Zhai<sup>33</sup>, Y. H. Zhan<sup>57</sup>, A. Q. Zhang<sup>1,61</sup>, B. L. Zhang<sup>1,61</sup>, B. X. Zhang<sup>1</sup>, D. H. Zhang<sup>42</sup>, G. Y. Zhang<sup>20</sup>, H. Zhang<sup>69</sup>, H. H. Zhang<sup>57</sup>, H. H. Zhang<sup>33</sup>, H. Q. Zhang<sup>1,56,61</sup>, H. Y. Zhang<sup>1,56</sup>, J. J. Zhang<sup>50</sup>, J. L. Zhang<sup>75</sup>, J. Q. Zhang<sup>40</sup>, J. W. Zhang<sup>1,56,61</sup>, J. X. Zhang<sup>37,j,k</sup>, J. Y. Zhang<sup>1</sup>, J. Z. Zhang<sup>1,61</sup>, Jiawei Zhang<sup>1,61</sup>, L. M. Zhang<sup>59</sup>, L. Q. Zhang<sup>57</sup>, Lei Zhang<sup>41</sup>, P. Zhang<sup>1</sup>, Q. Y. Zhang<sup>38,79</sup>, Shuihan Zhang<sup>1,61</sup>, Shulei Zhang<sup>25,h</sup>, X. D. Zhang<sup>44</sup>, X. M. Zhang<sup>1</sup>, X. Y. Zhang<sup>48</sup>, X. Y. Zhang<sup>53</sup>, Y. Zhang<sup>67</sup>, Y. T. Zhang<sup>79</sup>, Y. H. Zhang<sup>1,56</sup>, Yan Zhang<sup>69,56</sup>, Yao Zhang<sup>1</sup>, Z. H. Zhang<sup>1</sup>, Z. L. Zhang<sup>33</sup>, Z. Y. Zhang<sup>74</sup>, Z. Y. Zhang<sup>42</sup>, G. Zhao<sup>1</sup>, J. Zhao<sup>38</sup>, J. Y. Zhao<sup>1,61</sup>, J. Z. Zhao<sup>1,56</sup>, Lei Zhao<sup>69,56</sup>, Ling Zhao<sup>1</sup>, M. G. Zhao<sup>42</sup>, S. J. Zhao<sup>79</sup>, Y. B. Zhao<sup>1,56</sup>, Y. X. Zhao<sup>30,61</sup>, Z. G. Zhao<sup>69,56</sup>, A. Zhemchugov<sup>35,a</sup>, B. Zheng<sup>70</sup>, J. P. Zheng<sup>1,56</sup>, W. J. Zheng<sup>1,61</sup>, Y. H. Zheng<sup>61</sup>, B. Zhong<sup>40</sup>, X. Zhong<sup>57</sup>, H. Zhou<sup>48</sup>, L. P. Zhou<sup>1,61</sup>, X. Zhou<sup>74</sup>, X. R. Zhou<sup>69,56</sup>, X. Y. Zhou<sup>38</sup>, Y. Z. Zhou<sup>12,f</sup>, J. Zhu<sup>42</sup>, K. Zhu<sup>1</sup>, K. J. Zhu<sup>1,56,61</sup>, L. Zhu<sup>33</sup>, L. X. Zhu<sup>61</sup>, S. H. Zhu<sup>68</sup>, S. Q. Zhu<sup>41</sup>, T. J. Zhu<sup>12,f</sup>, W. J. Zhu<sup>12,f</sup>, Y. C. Zhu<sup>69,56</sup>, Z. A. Zhu<sup>1,61</sup>, J. H. Zou<sup>1</sup>, J. Zu<sup>69,56</sup>

(BESIII Collaboration)

<sup>1</sup> Institute of High Energy Physics, Beijing 100049, People's Republic of China

<sup>2</sup> Beihang University, Beijing 100191, People's Republic of China

<sup>3</sup> Beijing Institute of Petrochemical Technology, Beijing 102617, People's Republic of China

<sup>4</sup> Bochum Ruhr-University, D-44780 Bochum, Germany

<sup>5</sup> Carnegie Mellon University, Pittsburgh, Pennsylvania 15213, USA

<sup>6</sup> Central China Normal University, Wuhan 430079, People's Republic of China

<sup>7</sup> Central South University, Changsha 410083, People's Republic of China

<sup>8</sup> China Center of Advanced Science and Technology, Beijing 100190, People's Republic of China

<sup>9</sup> China University of Geosciences, Wuhan 430074, People's Republic of China

<sup>10</sup> Chung-Ang University, Seoul, 06974, Republic of Korea

<sup>11</sup> COMSATS University Islamabad, Lahore Campus, Defence Road, Off Raiwind Road, 54000 Lahore, Pakistan

<sup>12</sup> Fudan University, Shanghai 200433, People's Republic of China

<sup>13</sup> G.I. Budker Institute of Nuclear Physics SB RAS (BINP), Novosibirsk 630090, Russia

<sup>14</sup> GSI Helmholtzcentre for Heavy Ion Research GmbH, D-64291 Darmstadt, Germany

<sup>15</sup> Guangxi Normal University, Guilin 541004, People's Republic of China

<sup>16</sup> Guangxi University, Nanning 530004, People's Republic of China

<sup>17</sup> Hangzhou Normal University, Hangzhou 310036, People's Republic of China

<sup>18</sup> Hebei University, Baoding 071002, People's Republic of China

<sup>19</sup> Helmholtz Institute Mainz, Staudinger Weg 18, D-55099 Mainz, Germany

<sup>20</sup> Henan Normal University, Xinxiang 453007, People's Republic of China

<sup>21</sup> Henan University of Science and Technology, Luoyang 471003, People's Republic of China

<sup>22</sup> Henan University of Technology, Zhengzhou 450001, People's Republic of China

<sup>23</sup> Huangshan College, Huangshan 245000, People's Republic of China

<sup>24</sup> Hunan Normal University, Changsha 410081, People's Republic of China

<sup>25</sup> Hunan University, Changsha 410082, People's Republic of China

<sup>26</sup> Indian Institute of Technology Madras, Chennai 600036, India

<sup>27</sup> Indiana University, Bloomington, Indiana 47405, USA

<sup>28</sup> INFN Laboratori Nazionali di Frascati, (A)INFN Laboratori Nazionali di Frascati, I-00044, Frascati, Italy; (B)INFN Sezione di Perugia, I-06100, Perugia, Italy; (C)University of Perugia, I-06100, Perugia, Italy

<sup>29</sup> INFN Sezione di Ferrara, (A)INFN Sezione di Ferrara, I-44122, Ferrara, Italy; (B)University of Ferrara, I-44122, Ferrara, Italy

<sup>30</sup> Institute of Modern Physics, Lanzhou 730000, People's Republic of China

<sup>31</sup> Institute of Physics and Technology, Peace Avenue 54B, Ulaanbaatar 13330, Mongolia

<sup>32</sup> Instituto de Alta Investigación, Universidad de Tarapacá, Casilla 7D, Arica, Chile

<sup>33</sup> Jilin University, Changchun 130012, People's Republic of China

<sup>34</sup> Johannes Gutenberg University of Mainz, Johann-Joachim-Becher-Weg 45, D-55099 Mainz, Germany

<sup>35</sup> Joint Institute for Nuclear Research, 141980 Dubna, Moscow region, Russia

<sup>36</sup> Justus-Liebig-Universität Giessen, II. Physikalisches Institut, Heinrich-Buff-Ring 16, D-35392 Giessen, Germany

<sup>37</sup> Lanzhou University, Lanzhou 730000, People's Republic of China

<sup>38</sup> Liaoning Normal University, Dalian 116029, People's Republic of China

<sup>39</sup> Liaoning University, Shenyang 110036, People's Republic of China

<sup>40</sup> Nanjing Normal University, Nanjing 210023, People's Republic of China

<sup>41</sup> Nanjing University, Nanjing 210093, People's Republic of China

<sup>42</sup> Nankai University, Tianjin 300071, People's Republic of China

<sup>43</sup> National Centre for Nuclear Research, Warsaw 02-093, Poland

<sup>44</sup> North China Electric Power University, Beijing 102206, People's Republic of China

<sup>45</sup> Peking University, Beijing 100871, People's Republic of China

<sup>46</sup> Qufu Normal University, Qufu 273165, People's Republic of China

<sup>47</sup> Shandong Normal University, Jinan 250014, People's Republic of China

- <sup>48</sup> Shandong University, Jinan 250100, People's Republic of China
- <sup>49</sup> Shanghai Jiao Tong University, Shanghai 200240, People's Republic of China
- <sup>50</sup> Shanxi Normal University, Linfen 041004, People's Republic of China
- <sup>51</sup> Shanxi University, Taiyuan 030006, People's Republic of China
- <sup>52</sup> Sichuan University, Chengdu 610064, People's Republic of China
- <sup>53</sup> Soochow University, Suzhou 215006, People's Republic of China
- <sup>54</sup> South China Normal University, Guangzhou 510006, People's Republic of China
- <sup>55</sup> Southeast University, Nanjing 211100, People's Republic of China
- <sup>56</sup> State Key Laboratory of Particle Detection and Electronics, Beijing 100049, Hefei 230026, People's Republic of China
- <sup>57</sup> Sun Yat-Sen University, Guangzhou 510275, People's Republic of China
- <sup>58</sup> Suranaree University of Technology, University Avenue 111, Nakhon Ratchasima 30000, Thailand
- <sup>59</sup> Tsinghua University, Beijing 100084, People's Republic of China
- <sup>60</sup> Turkish Accelerator Center Particle Factory Group, (A)Istinye University, 34010, Istanbul, Turkey; (B)Near East University, Nicosia, North Cyprus, 99138, Mersin 10, Turkey
- <sup>61</sup> University of Chinese Academy of Sciences, Beijing 100049, People's Republic of China
- <sup>62</sup> University of Groningen, NL-9747 AA Groningen, The Netherlands
- <sup>63</sup> University of Hawaii, Honolulu, Hawaii 96822, USA
- <sup>64</sup> University of Jinan, Jinan 250022, People's Republic of China
- <sup>65</sup> University of Manchester, Oxford Road, Manchester, M13 9PL, United Kingdom
- <sup>66</sup> University of Muenster, Wilhelm-Klemm-Strasse 9, 48149 Muenster, Germany
- <sup>67</sup> University of Oxford, Keble Road, Oxford OX13RH, United Kingdom
- <sup>68</sup> University of Science and Technology Liaoning, Anshan 114051, People's Republic of China
- <sup>69</sup> University of Science and Technology of China, Hefei 230026, People's Republic of China
- <sup>70</sup> University of South China, Hengyang 421001, People's Republic of China
- <sup>71</sup> University of the Punjab, Lahore-54590, Pakistan
- <sup>72</sup> University of Turin and INFN, (A)University of Turin, I-10125, Turin, Italy; (B)University of Eastern Piedmont, I-15121, Alessandria, Italy; (C)INFN, I-10125, Turin, Italy
- <sup>73</sup> Uppsala University, Box 516, SE-75120 Uppsala, Sweden
- <sup>74</sup> Wuhan University, Wuhan 430072, People's Republic of China
- <sup>75</sup> Xinyang Normal University, Xinyang 464000, People's Republic of China
- <sup>76</sup> Yantai University, Yantai 264005, People's Republic of China
- <sup>77</sup> Yunnan University, Kunming 650500, People's Republic of China
- <sup>78</sup> Zhejiang University, Hangzhou 310027, People's Republic of China
- <sup>79</sup> Zhengzhou University, Zhengzhou 450001, People's Republic of China <sup>a</sup> Also at the Moscow Institute of Physics and Technology, Moscow 141700, Russia
- <sup>b</sup> Also at the Novosibirsk State University, Novosibirsk, 630090, Russia
- <sup>c</sup> Also at the NRC "Kurchatov Institute", PNPI, 188300, Gatchina, Russia
- <sup>d</sup> Also at Goethe University Frankfurt, 60323 Frankfurt am Main, Germany
- <sup>e</sup> Also at Key Laboratory for Particle Physics, Astrophysics and Cosmology, Ministry of Education; Shanghai Key Laboratory for Particle Physics and Cosmology; Institute of Nuclear and Particle Physics, Shanghai 200240, People's Republic of China
- <sup>f</sup> Also at Key Laboratory of Nuclear Physics and Ion-beam Application (MOE) and Institute of Modern Physics, Fudan University, Shanghai 200443, People's Republic of China
- <sup>g</sup> Also at State Key Laboratory of Nuclear Physics and Technology, Peking University, Beijing 100871, People's Republic of China
- <sup>h</sup> Also at School of Physics and Electronics, Hunan University, Changsha 410082, China
- <sup>i</sup> Also at Guangdong Provincial Key Laboratory of Nuclear Science, Institute of Quantum Matter, South China Normal University, Guangzhou 510006, China
- <sup>j</sup> Also at Frontiers Science Center for Rare Isotopes, Lanzhou University, Lanzhou 730000, People's Republic of China
- <sup>k</sup> Also at Lanzhou Center for Theoretical Physics, Lanzhou University, Lanzhou 730000, People's Republic of China
- <sup>l</sup> Also at the Department of Mathematical Sciences, IBA, Karachi, Pakistan

## Appendix A: MAXIMUM LIKELIHOOD FITTING

The predicted cross-section  $\sigma_i^{pred}$  at  $i$ -th bin for each category X (=A,B,C) can be obtained as below:

$$\sigma_i^{pred} = \int_{bin} \frac{d\sigma}{d\cos\theta} d\cos\theta, \quad (A1)$$

with the theoretical formula,

$$\frac{d\sigma}{d\cos\theta} = \frac{\pi\alpha^2\beta}{2s} |G_M|^2 (1 + \cos^2\theta + \tau R_{em}^2 \sin^2\theta), \quad (A2)$$

where  $\tau = \frac{4m_n^2}{s}$ ,  $|G_M|$  and  $R_{em} \equiv |G_E|/|G_M|$  are two free parameters shared by 3 categories to be determined with the following minimization.

We minimize a negative logarithm likelihood as below:

$$LL = -\log\left(\prod_{X=A,B,C} \prod_{i=1}^7 \frac{(N_{X,i}^{pred})^{N_{X,i}^{obs}} e^{-N_{X,i}^{pred}}}{N_{X,i}^{obs}!}\right) \quad (A3)$$

$$N_{X,i}^{pred} = \begin{cases} \mathcal{L}\sigma^{pred}(\mathcal{E}^{MC} C_{dm} C_{trg} (1 + \delta))_{A,i}, \\ \mathcal{L}\sigma^{pred}(\mathcal{E}^{MC} C_{dm} C_{trg} C_{muc} (1 + \delta))_{B,i}, \\ \mathcal{L}\sigma^{pred}(\mathcal{E}^{MC} C_{dm} C_{trg} C_{ee} C_{muc} (1 + \delta))_{C,i}, \end{cases} \quad (A4)$$

where  $N_{X,i}^{obs}$  and  $N_{X,i}^{pred}$  represent number of observed events and number of predicted events,  $\mathcal{L}$  is the luminosity,  $\mathcal{E}^{MC}$  is the signal efficiency, ( $C_{dm}$ ,  $C_{trg}$ ,  $C_{ee}$ ,  $C_{muc}$ ) are four types of efficiency corrections,  $(1 + \delta)$  is the initial-state-radiation and vacuum polarization correction determined by the signal MC generator, at  $i$ -th bin for category X.

The systematic uncertainty at each bin is calculated to be  $\Delta_{T,i} = \sqrt{\Delta_{uc,i}^2 + \Delta_{c,i}^2}$ , where  $\Delta_{uc} = N^{obs} * \sqrt{R_{dm}^2 + R_{isr}^2}$  represents the uncorrelated uncertainty, and  $\Delta_c = N^{obs} * R_c$  the correlated one. Here,  $R_c$  is the relative systematic uncertainties which are quoted from Ref. [1].  $R_{dm}$  is directly calculated with  $C_{dm}$  values, for example  $C_{dm} = 1.23 \pm 0.10$  yields a  $R_{dm} = \frac{0.10}{1.23}$ , so are the others.

Thus the negative logarithm likelihood becomes:

$$LL = -\log\left(\prod_{X=A,B,C} \prod_{i=1}^7 \int P_a \otimes P_b\right), \quad (A5)$$

$$P_a = \frac{(N_{X,i}^{pred})^{N_{X,i}^{obs}} e^{-N_{X,i}^{pred}}}{N_{X,i}^{obs}!}, \quad (A6)$$

$$P_b = e^{-\frac{1}{2} \left( \frac{N_{X,i}^{obs} - N_{X,i}^{pred}}{N_{X,i}^{obs} * R_{X,i}} \right)^2}, \quad (A7)$$

using a convolution between a Poisson probability ( $P_a$ ) and a Gaussian probability ( $P_b$ ) which describes the systematic uncertainties per bin per category.

## Appendix B: FITTING ELECTROMAGNETIC FORM FACTORS

Figures 6 illustrates the fitting to data of the effective form factors with the following formulas [1, 2]:

$$\begin{aligned} \mathcal{F}_0 &= A, \quad \mathcal{F}_1 = A + A_{osc} \exp(-B\gamma\beta\sqrt{q^2}) \times \cos(C\gamma\beta\sqrt{q^2} + D)(1 - q^2/0.71)^2, \\ \mathcal{F}_2 &= \frac{A}{1 + q^2/m_a^2}, \quad \mathcal{F}_3 = \frac{A}{1 + q^2/m_a^2} + A_{osc} \exp(-B\gamma\beta\sqrt{q^2}) \times \cos(C\gamma\beta\sqrt{q^2} + D)(1 - q^2/0.71)^2. \end{aligned} \quad (B1)$$

---

[1] M. Ablikim *et al.* (BESIII Collaboration), Nat. Phys. 17, 1200 (2021).

[2] A. Bianconi and E. Tomasi-Gustafsson, Phys. Rev. Lett. **114**, 232301 (2015).

### Appendix C: SYSTEMATIC UNCERTAINTIES

Tables II, III and IV lists systematic uncertainties of antineutron angular distributions per  $\cos\theta_{\bar{n}}$  bin at 12 c.m. energies for three categories: luminosity ( $U_L^A$ ), antineutron and neutron selections ( $U_{n,\bar{n}}^A$ ),  $T_0$  and  $T_0^n$  misalignment ( $U_{T_0}^A$ ), angular distribution ( $U_{model}^A$ ), antineutron and neutron misidentification ( $U_{mis}^A$ ), time resolution of the neutron ( $U_{res}^A$ ), event-level selections ( $U_{evt}^A$ ), signal yields extraction ( $U_{fit}^A$ ), Conexc generator iteration ( $U_{ISR}^A$ ), trigger efficiency ( $U_{tri}^A$ ). Table V lists values of  $R_{em} = |G_E|/|G_M|$ , electric  $|G_E|$  and magnetic  $|G_M|$  form factors together with their systematic uncertainties.

Two steps are performed to extract the free parameters, and their uncertainties. Firstly angular distributions of the antineutron are analyzed only considering the statistical uncertainties per bin. The values of  $R_{em}$  and  $|G_M|$  can be estimated directly using the open source packages: RooFit and TMinuit. Secondly angular distributions of the antineutron including the systematic uncertainties per bin are further analyzed. The values of  $R_{em}$  and  $G_M$  are obtained and compared to previous ones. The differences between central values obtained with/without including systematic uncertainties of angular distributions of the antineutron is also considered as a source of systematic uncertainty as summarized in Table V. From these numbers, the statistical uncertainties are dominant and the systematic uncertainties are much smaller than the statistical uncertainties, because main sources of systematic uncertainties are correlated among bins. Considering the relation  $\sigma \propto |G_M|^2 [(1 + \tau R_{em}^2) + (1 - \tau R_{em}^2) \cos^2 \theta_{\bar{n}}]$ , the power 2 means uncertainties of form factors are half discounted compared to uncertainties of cross sections of the process  $e^+e^- \rightarrow n\bar{n}$  after the error propagation. Since  $|G_E|$  is strongly anti-correlated to  $|G_M|$ , the uncertainties of  $|G_E|$  are estimated with both uncertainties of  $|G_M|$  and uncertainties of  $R_{em}$ , and values of the correlation coefficient between  $|G_M|$  and  $R_{em}$  in Table V in the error propagation. (Ref: [https://root.cern/download/doc/RooFit\\_Users\\_Manual.2.91-33.pdf](https://root.cern/download/doc/RooFit_Users_Manual.2.91-33.pdf))

TABLE II. Summary of all systematic uncertainty sources in Category A. The last column is the summary of the total uncertainties.

| $\sqrt{s}$ GeV | $U_L^A$ | $U_{n,\bar{n}}^A$ | $U_{T_0}^A$ | $U_{model}^A$ | $U_{mis}^A$ | $U_{res}^A$ | $U_{fit}^A$ | $U_{ISR1}^A$ | $U_{ISR2}^A$ | $U_{tri}^A$ | Total (%) |
|----------------|---------|-------------------|-------------|---------------|-------------|-------------|-------------|--------------|--------------|-------------|-----------|
| 2.0000         | 1.0     | 3.1               | 0.2         | 10.8          | 0.1         | 5.0         | 4.2         | 1.0          | 0.3          | 4.6         | 13.9      |
| 2.0500         | 1.0     | 2.7               | 0.2         | 10.3          | 0.1         | 5.0         | 3.5         | 1.0          | 0.6          | 4.6         | 13.2      |
| 2.1000         | 1.0     | 2.4               | 0.2         | 7.8           | 0.1         | 5.0         | 12.1        | 1.0          | 1.2          | 4.6         | 16.2      |
| 2.1500         | 1.0     | 2.3               | 0.2         | 9.5           | 0.1         | 5.0         | 4.0         | 1.0          | 1.4          | 4.6         | 12.7      |
| 2.1250         | 1.0     | 2.3               | 0.2         | 8.1           | 0.1         | 5.0         | 12.3        | 1.0          | 1.7          | 4.6         | 16.5      |
| 2.1750         | 1.0     | 2.2               | 0.2         | 8.8           | 0.1         | 5.0         | 10.9        | 1.0          | 1.8          | 4.6         | 15.9      |
| 2.2000         | 1.0     | 2.1               | 0.2         | 8.0           | 0.1         | 5.0         | 8.3         | 1.0          | 2.2          | 4.5         | 13.8      |
| 2.2324         | 1.0     | 2.1               | 0.2         | 8.0           | 0.1         | 5.0         | 8.8         | 1.0          | 2.2          | 4.5         | 14.1      |
| 2.3094         | 1.0     | 2.0               | 0.2         | 8.7           | 0.1         | 5.0         | 5.7         | 1.0          | 1.4          | 4.2         | 12.6      |
| 2.3864         | 1.0     | 1.8               | 0.2         | 9.0           | 0.1         | 5.0         | 2.8         | 1.0          | 1.6          | 4.1         | 11.8      |
| 2.3960         | 1.0     | 1.8               | 0.2         | 9.0           | 0.1         | 5.0         | 3.2         | 1.0          | 1.8          | 4.1         | 11.9      |
| 2.6440         | 1.0     | 1.4               | 0.2         | 5.1           | 0.1         | 5.0         | 11.0        | 1.0          | 1.6          | 3.0         | 13.7      |
| 2.9000         | 1.0     | 1.5               | 0.2         | 1.3           | 0.1         | 5.0         | 6.6         | 1.0          | 3.2          | 2.6         | 9.6       |
| 2.9500         | 1.0     | 1.5               | 0.2         | 1.3           | 0.1         | 5.0         | 81          | 1.0          | 3.7          | 2.6         | 81.3      |

TABLE III. Summary of all systematic uncertainty sources in Category B. The last column is the summary of the total uncertainties.

| $\sqrt{s}$ (GeV) | $U_{n\bar{n}}^B$ | $U_{evt}^B$ | $U_{BDT}^B$ | $U_{fit}^B$ | $U_{model}^B$ | $U_{trig}^B$ | $U_{ISR1}^B$ | $U_{ISR2}^B$ | $U_L^B$ | Total (%) |
|------------------|------------------|-------------|-------------|-------------|---------------|--------------|--------------|--------------|---------|-----------|
| 2.0000           | 3.3              | 6.6         | 6.0         | 3.1         | 5.2           | 5.1          | 1.0          | 0.3          | 1.0     | 12.5      |
| 2.0500           | 2.2              | 5.2         | 6.0         | 6.4         | 9.2           | 5.0          | 1.0          | 0.6          | 1.0     | 14.8      |
| 2.1000           | 1.7              | 5.4         | 6.0         | 0.4         | 9.6           | 4.6          | 1.0          | 1.2          | 1.0     | 13.6      |
| 2.1250           | 1.7              | 5.0         | 6.0         | 1.0         | 9.6           | 4.5          | 1.0          | 1.4          | 1.0     | 13.5      |
| 2.1500           | 1.5              | 6.4         | 3.8         | 1.6         | 9.6           | 4.3          | 1.0          | 1.7          | 1.0     | 13.4      |
| 2.1750           | 1.5              | 6.4         | 3.8         | 1.1         | 6.5           | 4.6          | 1.0          | 1.8          | 1.0     | 11.4      |
| 2.2000           | 1.3              | 6.5         | 3.8         | 0.8         | 10.3          | 4.2          | 1.0          | 2.2          | 1.0     | 13.8      |
| 2.2320           | 1.3              | 6.2         | 3.8         | 2.4         | 9.7           | 4.2          | 1.0          | 2.2          | 1.0     | 13.4      |
| 2.3090           | 1.3              | 6.4         | 3.8         | 1.4         | 8.5           | 3.2          | 1.0          | 1.4          | 1.0     | 12.1      |
| 2.3860           | 1.1              | 3.4         | 3.6         | 1.6         | 10.4          | 2.8          | 1.0          | 1.6          | 1.0     | 12.2      |
| 2.3960           | 1.1              | 3.4         | 3.6         | 0.6         | 7.1           | 3.1          | 1.0          | 1.8          | 1.0     | 9.6       |
| 2.6440           | 0.8              | 9.5         | 3.9         | 1.7         | 7.3           | 2.1          | 1.0          | 1.6          | 1.0     | 13.1      |
| 2.9000           | 0.6              | 9.5         | 4.8         | 1.5         | 7.3           | 1.7          | 1.0          | 3.2          | 1.0     | 13.6      |
| 2.9500           | 1.0              | 9.7         | 4.8         | 4.3         | 7.3           | 1.4          | 1.0          | 3.7          | 1.0     | 14.4      |

TABLE IV. Summary of all systematic uncertainty sources in Category C. The last column is the summary of the total uncertainties.

| $\sqrt{s}$ GeV | $\delta_L^C$ | $\delta_{\text{sel}}^C$ | $\delta_{\text{fit}}^C$ | $\delta_{\text{model}}^C$ | $\delta_{\text{trg}}^C$ | $\delta_{\text{ISR1}}^C$ | $\delta_{\text{ISR2}}^C$ | Total (%) |
|----------------|--------------|-------------------------|-------------------------|---------------------------|-------------------------|--------------------------|--------------------------|-----------|
| 2.0000         | 1.0          | 6.6                     | 11.8                    | 18.8                      | 5.3                     | 1.0                      | 0.3                      | 23.8      |
| 2.0500         | 1.0          | 4.1                     | 10.3                    | 16.8                      | 4.3                     | 1.0                      | 0.6                      | 20.6      |
| 2.1000         | 1.0          | 4.2                     | 9.5                     | 15.6                      | 4.0                     | 1.0                      | 1.2                      | 19.3      |
| 2.1250         | 1.0          | 3.2                     | 11.1                    | 10.0                      | 3.9                     | 1.0                      | 1.4                      | 15.9      |
| 2.1500         | 1.0          | 3.5                     | 15.5                    | 9.6                       | 3.8                     | 1.0                      | 1.7                      | 19.1      |
| 2.1750         | 1.0          | 3.9                     | 11.9                    | 8.3                       | 4.0                     | 1.0                      | 1.8                      | 15.7      |
| 2.2000         | 1.0          | 3.9                     | 11.4                    | 8.3                       | 3.8                     | 1.0                      | 2.2                      | 15.3      |
| 2.2324         | 1.0          | 3.1                     | 12.0                    | 9.2                       | 3.8                     | 1.0                      | 2.2                      | 16.1      |
| 2.3094         | 1.0          | 3.9                     | 6.4                     | 7.6                       | 2.9                     | 1.0                      | 1.4                      | 11.2      |
| 2.3864         | 1.0          | 3.4                     | 5.5                     | 6.3                       | 2.5                     | 1.0                      | 1.6                      | 9.6       |
| 2.3960         | 1.0          | 3.4                     | 7.2                     | 6.3                       | 2.5                     | 1.0                      | 1.8                      | 10.7      |
| 2.6454         | 1.0          | 3.5                     | 16.8                    | 9.8                       | 1.9                     | 1.0                      | 1.6                      | 20.0      |
| 2.9000         | 1.0          | 5.5                     | 11.9                    | 9.3                       | 1.7                     | 1.0                      | 3.2                      | 16.5      |
| 2.9500         | 1.0          | 6.4                     | 77.9                    | 12.2                      | 1.6                     | 1.0                      | 3.7                      | 79.2      |

TABLE V. The form factor ratios  $R_{em} = |G_E|/|G_M|$ , electric  $|G_E|$  and magnetic  $|G_M|$  form factors. The results are obtained by fitting angular distributions of the antineutron w/o systematic uncertainties at each bin. The center shifts of results w/o considering systematic uncertainties per  $\cos\theta_{\bar{n}}$  during the fitting is also taken as a systematic uncertainty added to final results. The label "stat. only" represents results obtained from the fitting to data of antineutron angular distributions with statistical errors. The label "stat. + sys." represents results obtained from the fitting to data of antineutron angular distributions with both statistical errors and systematic errors.

| $\sqrt{s}$ (GeV)             | $R_{em}$                 |              |              |                        |
|------------------------------|--------------------------|--------------|--------------|------------------------|
|                              | stat. only               | stat. + sys. | center shift | total sys. uncertainty |
| 2.0000,2.0500                | 0.74±0.69                | 0.93±0.78    | 0.19         | 0.40                   |
| 2.1250,2.1500                | 1.32±0.37                | 1.29±0.45    | 0.02         | 0.25                   |
| 2.1750,2.2000,2.2324, 2.3094 | 1.53±0.64                | 1.51±0.67    | 0.03         | 0.19                   |
| 2.3864,2.3960                | 0.89±0.34                | 0.88±0.38    | 0.02         | 0.16                   |
| 2.6454,2.9500                | 0.90±0.77                | 0.56±0.99    | 0.34         | 0.70                   |
| $\sqrt{s}$ ( GeV)            | $ G_M $ ( $10^{-2}$ )    |              |              |                        |
|                              | stat. only               | stat. + sys. | center shift | total sys. uncertainty |
| 2.0000,2.0500                | 20.3±5.0                 | 18.6±5.6     | 1.8          | 3.1                    |
| 2.1250,2.1500                | 8.7±1.2                  | 8.7±1.5      | 0.0          | 0.8                    |
| 2.1750,2.2000,2.2324, 2.3094 | 6.6±1.5                  | 6.5±1.6      | 0.1          | 0.4                    |
| 2.3864,2.3960                | 8.4±0.9                  | 8.3±0.9      | 0.0          | 0.4                    |
| 2.6454,2.9500                | 4.2±0.8                  | 4.4±0.9      | 0.2          | 0.3                    |
| $\sqrt{s}$ ( GeV)            | $ G_E $ ( $10^{-2}$ )    |              |              |                        |
|                              | correlation coefficients | stat. only   | center shift | total uncertainty      |
| 2.0000,2.0500                | -0.984                   | 17.2±8.3     | -            | 4.7                    |
| 2.1250,2.1500                | -0.990                   | 11.2±1.7     | -            | 1.1                    |
| 2.1750,2.2000,2.2324, 2.3094 | -0.992                   | 9.8±1.9      | -            | 0.6                    |
| 2.3864,2.3960                | -0.979                   | 7.3±2.1      | -            | 1.0                    |
| 2.6454,2.9500                | -0.968                   | 2.5±2.9      | -            | 2.9                    |

# Appendix D: DATA

TABLE VI. Differential cross-sections for category A, in unit of pb.

| $\sqrt{s}$ GeV | bin1                           | bin2                           | bin3                           | bin4                           | bin5                           | bin6                            | bin7                           |
|----------------|--------------------------------|--------------------------------|--------------------------------|--------------------------------|--------------------------------|---------------------------------|--------------------------------|
| 2.0000         | $18.9^{+12.9}_{-9.7} \pm 3.0$  | $35.4^{+18.0}_{-14.3} \pm 3.0$ | $30.2^{+14.0}_{-11.0} \pm 3.0$ | $37.3^{+21.4}_{-17.1} \pm 3.0$ | $29.9^{+16.4}_{-13.3} \pm 3.0$ | $30.9^{+15.9}_{-12.5} \pm 3.0$  | $26.4^{+14.9}_{-11.4} \pm 3.0$ |
| 2.0500         | $0.0^{+30.3}_{-0.0} \pm 0.0$   | $0.0^{+7.2}_{-0.0} \pm 0.0$    | $42.9^{+30.5}_{-21.2} \pm 0.0$ | $16.7^{+37.0}_{-21.1} \pm 0.0$ | $12.7^{+25.3}_{-19.5} \pm 0.0$ | $100.0^{+44.5}_{-35.0} \pm 0.0$ | $25.2^{+24.9}_{-16.9} \pm 0.0$ |
| 2.1250         | $9.4^{+2.3}_{-2.0} \pm 1.3$    | $16.7^{+3.2}_{-2.8} \pm 1.3$   | $16.6^{+3.5}_{-3.2} \pm 1.3$   | $17.8^{+4.0}_{-3.6} \pm 1.3$   | $14.3^{+3.4}_{-3.0} \pm 1.3$   | $12.7^{+2.8}_{-2.6} \pm 1.3$    | $12.4^{+2.6}_{-2.3} \pm 1.3$   |
| 2.1500         | $15.2^{+22.4}_{-11.5} \pm 2.5$ | $16.1^{+26.9}_{-16.1} \pm 2.5$ | $0.0^{+9.9}_{-0.0} \pm 2.5$    | $29.0^{+49.8}_{-26.6} \pm 2.5$ | $0.0^{+10.5}_{-0.0} \pm 2.5$   | $51.4^{+38.1}_{-26.3} \pm 2.5$  | $0.0^{+7.8}_{-0.0} \pm 2.5$    |
| 2.1750         | $9.1^{+8.8}_{-5.5} \pm 1.5$    | $13.9^{+10.5}_{-7.2} \pm 1.5$  | $0.0^{+5.5}_{-0.0} \pm 1.5$    | $30.8^{+20.2}_{-16.0} \pm 1.5$ | $8.7^{+11.4}_{-7.2} \pm 1.5$   | $12.8^{+10.0}_{-6.9} \pm 1.5$   | $0.8^{+7.1}_{-0.0} \pm 1.5$    |
| 2.2200         | $2.8^{+5.4}_{-0.0} \pm 0.4$    | $6.9^{+8.4}_{-5.3} \pm 0.4$    | $0.0^{+2.7}_{-0.0} \pm 0.4$    | $18.9^{+12.3}_{-9.3} \pm 0.4$  | $7.6^{+7.5}_{-4.9} \pm 0.4$    | $0.9^{+8.2}_{-0.0} \pm 0.4$     | $2.9^{+5.0}_{-2.7} \pm 0.4$    |
| 2.2324         | $3.6^{+5.3}_{-2.7} \pm 0.5$    | $3.3^{+7.4}_{-2.2} \pm 0.5$    | $13.8^{+13.0}_{-9.0} \pm 0.5$  | $1.5^{+9.1}_{-1.1} \pm 0.5$    | $16.1^{+11.4}_{-8.2} \pm 0.5$  | $0.0^{+3.9}_{-0.0} \pm 0.5$     | $9.5^{+8.5}_{-5.9} \pm 0.5$    |
| 2.3094         | $3.7^{+4.4}_{-2.7} \pm 0.5$    | $14.0^{+6.8}_{-5.2} \pm 0.5$   | $17.5^{+9.5}_{-7.3} \pm 0.5$   | $8.2^{+8.7}_{-6.4} \pm 0.5$    | $13.3^{+7.6}_{-5.8} \pm 0.5$   | $11.1^{+8.2}_{-6.3} \pm 0.5$    | $4.5^{+6.0}_{-4.4} \pm 0.5$    |
| 2.3864         | $8.6^{+4.0}_{-4.0} \pm 1.1$    | $11.3^{+4.8}_{-3.1} \pm 1.1$   | $3.2^{+4.7}_{-3.1} \pm 1.1$    | $11.5^{+7.4}_{-5.8} \pm 1.1$   | $3.6^{+5.4}_{-3.5} \pm 1.1$    | $15.2^{+7.7}_{-6.0} \pm 1.1$    | $7.4^{+5.4}_{-4.1} \pm 1.1$    |
| 2.3960         | $10.2^{+2.8}_{-2.4} \pm 1.3$   | $10.6^{+3.4}_{-2.9} \pm 1.3$   | $6.8^{+3.0}_{-2.4} \pm 1.3$    | $14.7^{+4.8}_{-4.1} \pm 1.3$   | $7.0^{+3.4}_{-2.8} \pm 1.3$    | $9.6^{+3.2}_{-2.7} \pm 1.3$     | $9.8^{+2.9}_{-2.5} \pm 1.3$    |
| 2.6450         | $3.2^{+2.1}_{-1.5} \pm 0.5$    | $2.6^{+2.3}_{-1.4} \pm 0.5$    | $0.0^{+0.6}_{-0.0} \pm 0.5$    | $9.9^{+4.8}_{-3.7} \pm 0.5$    | $4.3^{+2.8}_{-2.0} \pm 0.5$    | $3.0^{+2.8}_{-1.9} \pm 0.5$     | $3.9^{+2.3}_{-1.7} \pm 0.5$    |
| 2.9500         | $0.0^{+1.8}_{-0.0} \pm 0.0$    | $0.0^{+1.8}_{-0.0} \pm 0.0$    | $0.0^{+2.5}_{-0.0} \pm 0.0$    | $0.0^{+2.8}_{-0.0} \pm 0.0$    | $2.4^{+6.5}_{-2.4} \pm 0.0$    | $4.2^{+6.7}_{-4.2} \pm 0.0$     | $0.0^{+1.6}_{-0.0} \pm 0.0$    |

TABLE VII. Differential cross-sections for category B, in unit of pb.

| $\sqrt{s}$ GeV | bin1                           | bin2                           | bin3                           | bin4                           | bin5                           | bin6                          | bin7                           |
|----------------|--------------------------------|--------------------------------|--------------------------------|--------------------------------|--------------------------------|-------------------------------|--------------------------------|
| 2.0000         | $24.8^{+46.0}_{-18.8} \pm 3.1$ | $75.3^{+68.2}_{-39.2} \pm 3.1$ | $45.8^{+60.5}_{-29.6} \pm 3.1$ | $38.7^{+63.9}_{-27.8} \pm 3.1$ | $55.5^{+73.3}_{-35.8} \pm 3.1$ | $0.0^{+26.4}_{-0.0} \pm 3.1$  | $55.1^{+61.3}_{-32.4} \pm 3.1$ |
| 2.0500         | $0.0^{+50.1}_{-0.0} \pm 0.0$   | $55.6^{+83.1}_{-38.3} \pm 0.0$ | $0.0^{+34.7}_{-0.0} \pm 0.0$   | $0.0^{+34.2}_{-0.0} \pm 0.0$   | $0.0^{+35.7}_{-0.0} \pm 0.0$   | $0.0^{+33.2}_{-0.0} \pm 0.0$  | $0.0^{+46.7}_{-0.0} \pm 0.0$   |
| 2.1250         | $10.9^{+3.1}_{-2.5} \pm 1.5$   | $13.6^{+2.8}_{-2.3} \pm 1.5$   | $12.7^{+2.7}_{-2.2} \pm 1.5$   | $11.6^{+2.6}_{-2.1} \pm 1.5$   | $10.1^{+2.5}_{-2.0} \pm 1.5$   | $9.3^{+2.4}_{-2.0} \pm 1.5$   | $14.5^{+3.4}_{-2.8} \pm 1.5$   |
| 2.1500         | $20.9^{+38.8}_{-15.9} \pm 3.0$ | $38.6^{+38.5}_{-21.3} \pm 3.0$ | $35.6^{+34.6}_{-19.3} \pm 3.0$ | $0.0^{+13.0}_{-0.0} \pm 3.0$   | $16.2^{+30.0}_{-12.3} \pm 3.0$ | $11.3^{+28.3}_{-9.6} \pm 3.0$ | $42.4^{+45.8}_{-24.6} \pm 3.0$ |
| 2.1750         | $14.0^{+12.1}_{-7.1} \pm 1.7$  | $9.4^{+9.4}_{-5.2} \pm 1.7$    | $13.0^{+10.1}_{-6.1} \pm 1.7$  | $10.2^{+9.5}_{-5.4} \pm 1.7$   | $6.4^{+8.5}_{-4.1} \pm 1.7$    | $6.8^{+8.9}_{-4.4} \pm 1.7$   | $10.5^{+12.5}_{-6.4} \pm 1.7$  |
| 2.2200         | $8.3^{+4.5}_{-4.5} \pm 1.2$    | $4.1^{+3.8}_{-2.7} \pm 1.2$    | $4.7^{+3.9}_{-3.0} \pm 1.2$    | $2.9^{+5.4}_{-3.9} \pm 1.2$    | $7.5^{+4.3}_{-3.9} \pm 1.2$    | $3.6^{+4.1}_{-2.6} \pm 1.2$   | $20.3^{+10.5}_{-6.4} \pm 1.2$  |
| 2.2324         | $0.0^{+3.2}_{-0.0} \pm 0.0$    | $0.5^{+4.9}_{-0.5} \pm 0.0$    | $9.0^{+7.7}_{-4.5} \pm 0.0$    | $16.4^{+9.2}_{-6.2} \pm 0.0$   | $10.5^{+8.2}_{-5.0} \pm 0.0$   | $11.1^{+5.1}_{-5.1} \pm 0.0$  | $15.1^{+10.6}_{-6.7} \pm 0.0$  |
| 2.3094         | $4.4^{+4.4}_{-2.4} \pm 0.6$    | $6.6^{+4.7}_{-2.9} \pm 0.6$    | $7.2^{+4.8}_{-3.1} \pm 0.6$    | $11.1^{+5.5}_{-3.9} \pm 0.6$   | $13.2^{+5.8}_{-4.2} \pm 0.6$   | $5.2^{+4.3}_{-2.5} \pm 0.6$   | $8.7^{+5.7}_{-3.7} \pm 0.6$    |
| 2.3864         | $4.2^{+3.5}_{-2.1} \pm 0.5$    | $10.0^{+4.1}_{-3.0} \pm 0.5$   | $10.0^{+4.2}_{-3.1} \pm 0.5$   | $6.2^{+3.6}_{-2.4} \pm 0.5$    | $6.0^{+3.4}_{-2.3} \pm 0.5$    | $12.7^{+4.5}_{-3.4} \pm 0.5$  | $7.1^{+4.0}_{-2.7} \pm 0.5$    |
| 2.3960         | $9.0^{+2.3}_{-1.8} \pm 0.8$    | $7.9^{+2.0}_{-1.6} \pm 0.8$    | $7.6^{+1.9}_{-1.6} \pm 0.8$    | $8.6^{+2.1}_{-1.7} \pm 0.8$    | $6.9^{+1.8}_{-1.5} \pm 0.8$    | $8.7^{+2.0}_{-1.7} \pm 0.8$   | $10.2^{+2.4}_{-2.0} \pm 0.8$   |
| 2.6450         | $2.6^{+1.1}_{-0.8} \pm 0.4$    | $1.4^{+0.9}_{-0.6} \pm 0.4$    | $2.2^{+1.0}_{-0.7} \pm 0.4$    | $2.4^{+1.1}_{-0.8} \pm 0.4$    | $1.4^{+0.9}_{-0.6} \pm 0.4$    | $2.2^{+1.0}_{-0.7} \pm 0.4$   | $2.2^{+1.1}_{-0.8} \pm 0.4$    |

TABLE VIII. Differential cross-sections for category C, in unit of pb.

| $\sqrt{s}$ GeV | bin1                            | bin2                            | bin3                           | bin4                            | bin5                            | bin6                            | bin7                            |
|----------------|---------------------------------|---------------------------------|--------------------------------|---------------------------------|---------------------------------|---------------------------------|---------------------------------|
| 2.0000         | $93.8^{+75.5}_{-45.5} \pm 24.4$ | $22.1^{+38.5}_{-16.4} \pm 24.4$ | $0.0^{+14.2}_{-0.0} \pm 24.4$  | $14.8^{+41.2}_{-13.0} \pm 24.4$ | $23.1^{+40.2}_{-17.2} \pm 24.4$ | $72.2^{+48.8}_{-31.2} \pm 24.4$ | $92.0^{+53.1}_{-35.6} \pm 24.4$ |
| 2.0500         | $54.3^{+69.0}_{-34.4} \pm 12.1$ | $19.7^{+45.2}_{-16.3} \pm 12.1$ | $0.0^{+19.9}_{-0.0} \pm 12.1$  | $73.4^{+68.1}_{-38.8} \pm 12.1$ | $0.0^{+19.2}_{-0.0} \pm 12.1$   | $8.0^{+40.8}_{-7.8} \pm 12.1$   | $48.4^{+59.4}_{-30.1} \pm 12.1$ |
| 2.1250         | $10.3^{+2.3}_{-1.9} \pm 1.7$    | $9.0^{+1.9}_{-1.6} \pm 1.7$     | $9.2^{+1.8}_{-1.6} \pm 1.7$    | $7.8^{+1.9}_{-1.6} \pm 1.7$     | $8.4^{+1.8}_{-1.5} \pm 1.7$     | $12.4^{+2.2}_{-1.9} \pm 1.7$    | $8.6^{+2.0}_{-1.6} \pm 1.7$     |
| 2.1500         | $9.6^{+2.0}_{-1.9} \pm 1.9$     | $0.0^{+8.9}_{-0.0} \pm 1.9$     | $27.3^{+26.6}_{-14.8} \pm 1.9$ | $19.5^{+25.7}_{-12.6} \pm 1.9$  | $7.3^{+20.3}_{-6.4} \pm 1.9$    | $0.0^{+8.4}_{-0.0} \pm 1.9$     | $0.0^{+8.9}_{-0.0} \pm 1.9$     |
| 2.1750         | $7.4^{+7.0}_{-3.9} \pm 1.2$     | $6.5^{+6.0}_{-3.4} \pm 1.2$     | $2.1^{+4.9}_{-1.8} \pm 1.2$    | $12.3^{+8.5}_{-5.4} \pm 1.2$    | $4.5^{+5.8}_{-2.9} \pm 1.2$     | $12.0^{+8.0}_{-5.1} \pm 1.2$    | $4.9^{+6.3}_{-3.1} \pm 1.2$     |
| 2.2200         | $6.1^{+5.3}_{-3.1} \pm 1.0$     | $7.9^{+5.1}_{-3.3} \pm 1.0$     | $10.9^{+6.1}_{-4.1} \pm 1.0$   | $1.1^{+3.3}_{-1.0} \pm 1.0$     | $2.3^{+3.9}_{-1.7} \pm 1.0$     | $15.2^{+6.3}_{-4.6} \pm 1.0$    | $5.9^{+4.8}_{-2.9} \pm 1.0$     |
| 2.2324         | $3.1^{+4.4}_{-2.1} \pm 0.5$     | $6.3^{+5.1}_{-3.1} \pm 0.5$     | $5.0^{+4.7}_{-2.7} \pm 0.5$    | $8.2^{+6.2}_{-3.8} \pm 0.5$     | $1.3^{+3.6}_{-1.2} \pm 0.5$     | $10.6^{+5.0}_{-4.0} \pm 0.5$    | $5.6^{+5.0}_{-2.9} \pm 0.5$     |
| 2.3094         | $12.4^{+4.6}_{-3.5} \pm 1.5$    | $7.4^{+3.7}_{-2.6} \pm 1.5$     | $0.6^{+2.1}_{-0.5} \pm 1.5$    | $3.5^{+3.3}_{-1.9} \pm 1.5$     | $7.7^{+3.9}_{-2.7} \pm 1.5$     | $11.4^{+4.2}_{-3.2} \pm 1.5$    | $1.6^{+2.4}_{-1.2} \pm 1.5$     |
| 2.3864         | $9.2^{+3.8}_{-2.8} \pm 1.0$     | $3.6^{+2.6}_{-1.4} \pm 1.0$     | $9.7^{+3.8}_{-2.8} \pm 1.0$    | $5.4^{+2.1}_{-1.6} \pm 1.0$     | $3.5^{+2.6}_{-1.6} \pm 1.0$     | $4.6^{+2.6}_{-1.8} \pm 1.0$     | $6.7^{+3.2}_{-2.2} \pm 1.0$     |
| 2.3960         | $6.2^{+1.7}_{-1.4} \pm 0.7$     | $4.4^{+1.4}_{-1.1} \pm 0.7$     | $7.9^{+1.8}_{-1.5} \pm 0.7$    | $6.0^{+1.6}_{-1.3} \pm 0.7$     | $7.2^{+1.7}_{-1.4} \pm 0.7$     | $7.9^{+1.7}_{-1.4} \pm 0.7$     | $8.4^{+1.8}_{-1.5} \pm 0.7$     |
| 2.6450         | $1.1^{+0.7}_{-0.5} \pm 0.3$     | $1.0^{+0.6}_{-0.4} \pm 0.3$     | $2.1^{+0.8}_{-0.6} \pm 0.3$    | $0.2^{+0.5}_{-0.2} \pm 0.3$     | $0.3^{+0.8}_{-0.2} \pm 0.3$     | $2.0^{+0.8}_{-0.6} \pm 0.3$     | $0.8^{+0.6}_{-0.4} \pm 0.3$     |
| 2.9500         | $0.0^{+0.6}_{-0.0} \pm 0.0$     | $0.0^{+0.6}_{-0.0} \pm 0.0$     | $0.0^{+0.6}_{-0.0} \pm 0.0$    | $2.5^{+2.2}_{-1.3} \pm 0.0$     | $1.0^{+1.7}_{-0.8} \pm 0.0$     | $1.9^{+1.7}_{-1.0} \pm 0.0$     | $0.0^{+0.6}_{-0.0} \pm 0.0$     |

TABLE IX. DATA:  $N_{signal}$  @CatA

| $\sqrt{s}$ | BIN1 | errL | errH | BIN2 | errL | errH | BIN3 | errL | errH | BIN4 | errL | errH | BIN5 | errL | errH | BIN6 | errL | errH | BIN7 | errL | errH | tot   |
|------------|------|------|------|------|------|------|------|------|------|------|------|------|------|------|------|------|------|------|------|------|------|-------|
| 2.0000     | 4.3  | 2.2  | 2.9  | 6.6  | 2.7  | 3.4  | 7.0  | 2.5  | 3.3  | 6.3  | 2.9  | 3.6  | 6.5  | 2.9  | 3.6  | 6.4  | 2.6  | 3.3  | 5.7  | 2.5  | 3.2  | 47.1  |
| 2.0500     | 0    | 0    | 2.1  | 0    | 0    | 0.5  | 3.2  | 1.6  | 2.3  | 1.0  | 0    | 2.1  | 0.7  | 0    | 1.4  | 7.3  | 2.5  | 3.2  | 2.2  | 1.5  | 2.2  | 14.4  |
| 2.1250     | 22.8 | 5.0  | 5.7  | 37.6 | 6.4  | 7.1  | 32.4 | 6.2  | 6.9  | 34.2 | 6.9  | 7.7  | 29.2 | 6.2  | 6.9  | 28.6 | 5.8  | 6.4  | 30.2 | 5.7  | 6.5  | 237.8 |
| 2.1500     | 0.9  | 0.7  | 1.4  | 1.0  | 1.0  | 1.6  | 0    | 0    | 0.5  | 1.3  | 0    | 2.2  | 0    | 0    | 0.5  | 3.3  | 1.7  | 2.4  | 0    | 0    | 0.5  | 7.4   |
| 2.1750     | 1.9  | 1.2  | 1.9  | 2.8  | 1.5  | 2.1  | 0    | 0    | 1.0  | 5.3  | 2.8  | 3.5  | 1.4  | 1.2  | 1.9  | 2.7  | 1.5  | 2.2  | 0.2  | 0    | 1.5  | 16.2  |
| 2.2000     | 0.8  | 0    | 1.5  | 1.6  | 1.2  | 1.9  | 0    | 0    | 0.6  | 4.2  | 2.0  | 2.7  | 2.1  | 1.3  | 2.0  | 0.2  | 0    | 2.1  | 0.8  | 0.8  | 1.4  | 10.5  |
| 2.2324     | 1.0  | 0.7  | 1.4  | 0.8  | 0    | 1.7  | 2.6  | 1.7  | 2.5  | 0.3  | 0    | 1.7  | 3.4  | 1.8  | 2.4  | 0    | 0    | 0.8  | 2.7  | 1.7  | 2.4  | 11.8  |
| 2.3094     | 1.5  | 1.1  | 1.8  | 5.9  | 2.2  | 2.9  | 6.0  | 2.5  | 3.3  | 2.7  | 2.1  | 2.9  | 5.2  | 2.3  | 3.0  | 4.5  | 2.6  | 3.3  | 2.2  | 2.1  | 2.9  | 29.5  |
| 2.3864     | 4.6  | 2.1  | 2.8  | 5.0  | 2.1  | 2.8  | 1.5  | 1.4  | 2.2  | 5.2  | 2.6  | 3.4  | 1.4  | 2.1  | 2.2  | 7.3  | 2.9  | 3.7  | 4.1  | 2.2  | 3    | 33.7  |
| 2.3960     | 16.5 | 3.8  | 4.5  | 14.1 | 3.9  | 4.6  | 9.4  | 3.4  | 4.2  | 17.5 | 5.0  | 5.7  | 8.7  | 3.5  | 4.2  | 13.9 | 3.9  | 4.6  | 15.3 | 3.9  | 4.6  | 111.9 |
| 2.6454     | 3.5  | 1.6  | 2.3  | 2.0  | 1.1  | 1.8  | 0    | 0    | 0.5  | 6.1  | 2.3  | 3.0  | 3.5  | 1.6  | 2.3  | 2.5  | 1.6  | 2.3  | 4.0  | 1.7  | 2.4  | 25.1  |
| 2.9500     | 0    | 0    | 0.5  | 0    | 0    | 0.5  | 0    | 0    | 0.5  | 0    | 0    | 0.5  | 0.5  | 0    | 1.4  | 1.1  | 1.1  | 1.8  | 0    | 0    | 0.5  | 0     |

TABLE X. DATA:  $N_{signal}$  @CatB

| $\sqrt{s}$ | BIN1 | errL | errH | BIN2 | errL | errH | BIN3 | errL | errH | BIN4 | errL | errH | BIN5 | errL | errH | BIN6 | errL | errH | BIN7 | errL | errH | tot   |
|------------|------|------|------|------|------|------|------|------|------|------|------|------|------|------|------|------|------|------|------|------|------|-------|
| 2.0000     | 1.3  | 1.0  | 2.4  | 3.3  | 1.7  | 3.0  | 2.0  | 1.3  | 2.6  | 1.5  | 1.1  | 2.5  | 2.0  | 1.3  | 2.6  | 0    | 0    | 1.0  | 2.5  | 1.5  | 2.8  | 12.8  |
| 2.0500     | 0    | 0    | 1.0  | 1.7  | 1.2  | 2.5  | 0    | 0    | 1.0  | 0    | 0    | 1.0  | 0    | 0    | 1.0  | 0    | 0    | 1.0  | 0    | 0    | 1.0  | 1.7   |
| 2.1250     | 19.3 | 4.4  | 5.5  | 33.6 | 5.8  | 6.9  | 31.4 | 5.6  | 6.7  | 28.8 | 5.3  | 6.4  | 24.6 | 4.9  | 6.0  | 22.2 | 4.7  | 5.8  | 25.9 | 5.1  | 6.2  | 205.0 |
| 2.1500     | 1.3  | 1.0  | 2.4  | 2.9  | 1.6  | 2.9  | 3.0  | 1.6  | 2.9  | 0    | 0    | 1.0  | 1.3  | 1.0  | 2.4  | 0.9  | 0.8  | 2.3  | 2.6  | 1.5  | 2.8  | 12.2  |
| 2.1750     | 3.5  | 1.8  | 3.0  | 2.9  | 1.6  | 2.9  | 4.1  | 1.9  | 3.2  | 3.2  | 1.7  | 3.0  | 2.0  | 1.3  | 2.6  | 2.0  | 1.3  | 2.6  | 2.3  | 1.4  | 2.7  | 23.5  |
| 2.2000     | 3.0  | 1.6  | 2.9  | 1.8  | 1.2  | 2.6  | 2.1  | 1.3  | 2.7  | 1.3  | 1.0  | 2.41 | 3.3  | 1.7  | 3.0  | 1.6  | 1.1  | 2.5  | 7.4  | 2.7  | 3.8  | 23.5  |
| 2.2324     | 0    | 0    | 1.0  | 0.2  | 0.2  | 2.0  | 3.6  | 1.8  | 3.1  | 6.6  | 2.5  | 3.7  | 4.1  | 1.9  | 3.2  | 4.3  | 2.0  | 3.2  | 4.7  | 2.1  | 3.3  | 23.5  |
| 2.3094     | 2.9  | 1.6  | 2.9  | 4.7  | 2.1  | 3.3  | 5.1  | 2.2  | 3.4  | 7.9  | 2.8  | 3.9  | 9.6  | 3.0  | 4.2  | 3.8  | 1.9  | 3.12 | 5.2  | 2.21 | 3.4  | 42.1  |
| 2.3864     | 3.7  | 1.8  | 3.1  | 10.6 | 3.2  | 4.4  | 10.3 | 3.2  | 4.3  | 6.1  | 2.4  | 3.6  | 6.5  | 2.5  | 3.7  | 13.3 | 3.6  | 4.7  | 6.5  | 2.5  | 3.7  | 60.7  |
| 2.3960     | 23.7 | 4.8  | 5.9  | 23.7 | 4.8  | 5.9  | 22.7 | 4.7  | 5.8  | 25.8 | 5.1  | 6.1  | 21.7 | 4.6  | 5.7  | 26.7 | 5.1  | 6.2  | 26.7 | 5.1  | 6.2  | 195.0 |
| 2.6454     | 9.5  | 3.0  | 4.2  | 5.9  | 2.4  | 3.6  | 8.6  | 2.9  | 4.1  | 9.3  | 3.0  | 4.2  | 5.8  | 2.3  | 3.5  | 9.0  | 2.9  | 4.1  | 7.9  | 2.8  | 3.9  | 65.5  |
| 2.9500     | 0    | 0    | 1.0  | 1.0  | 0.8  | 2.3  | 0    | 0    | 1.0  | 0    | 0    | 1.0  | 0    | 0    | 1.0  | 1.0  | 0.8  | 2.3  | 4.1  | 1.9  | 3.2  | 6.1   |

TABLE XI. DATA:  $N_{signal}$  @CatC

| $\sqrt{s}$ | BIN1 | errL | errH | BIN2 | errL | errH | BIN3 | errL | errH | BIN4 | errL | errH | BIN5 | errL | errH | BIN6 | errL | errH | BIN7 | errL | errH | tot   |
|------------|------|------|------|------|------|------|------|------|------|------|------|------|------|------|------|------|------|------|------|------|------|-------|
| 2.0000     | 3.9  | 1.9  | 3.1  | 1.4  | 1.0  | 2.4  | 0    | 0    | 1.0  | 0.8  | 0.7  | 2.2  | 1.4  | 1.0  | 2.4  | 5.0  | 2.2  | 3.4  | 6.3  | 2.4  | 3.6  | 18.8  |
| 2.0500     | 2.1  | 1.3  | 2.7  | 1.0  | 0.8  | 2.3  | 0    | 0    | 1.0  | 3.2  | 1.7  | 3.0  | 0    | 0    | 1.0  | 0.4  | 0.4  | 2.1  | 2.2  | 1.4  | 2.7  | 8.9   |
| 2.1250     | 29.7 | 5.4  | 6.5  | 32.7 | 5.7  | 6.8  | 34.6 | 5.9  | 6.9  | 24.5 | 4.9  | 6.0  | 31.4 | 5.6  | 6.7  | 43.7 | 6.6  | 7.7  | 27.7 | 5.2  | 6.3  | 254.0 |
| 2.1500     | 0.9  | 0.8  | 2.3  | 0    | 0    | 1.0  | 3.0  | 1.6  | 2.9  | 2.0  | 1.3  | 2.6  | 0.8  | 0.7  | 2.2  | 0    | 0    | 1.0  | 0    | 0    | 1.0  | 6.7   |
| 2.1750     | 3.1  | 1.7  | 2.9  | 3.2  | 1.7  | 3.0  | 1.0  | 0.8  | 2.3  | 4.9  | 2.1  | 3.4  | 2.1  | 1.3  | 2.7  | 5.1  | 2.2  | 3.4  | 2.1  | 1.3  | 2.7  | 24.6  |
| 2.2000     | 3.5  | 1.8  | 3.0  | 5.3  | 2.2  | 3.4  | 6.6  | 2.5  | 3.7  | 0.7  | 0.6  | 2.2  | 1.5  | 1.1  | 2.5  | 10.5 | 3.2  | 4.3  | 3.9  | 1.9  | 3.1  | 35.5  |
| 2.2324     | 1.8  | 1.2  | 2.6  | 3.9  | 1.9  | 3.1  | 3.1  | 1.7  | 2.9  | 4.3  | 2.0  | 3.2  | 0.8  | 0.7  | 2.2  | 6.8  | 2.5  | 3.7  | 3.4  | 1.8  | 3.0  | 25.9  |
| 2.3094     | 12.4 | 3.5  | 4.6  | 7.8  | 2.7  | 3.9  | 0.6  | 0.6  | 2.1  | 3.1  | 1.7  | 2.9  | 7.6  | 2.7  | 3.9  | 12.7 | 3.5  | 4.7  | 1.7  | 1.2  | 2.5  | 58.3  |
| 2.3864     | 10.5 | 3.2  | 4.3  | 4.5  | 2.0  | 3.3  | 11.6 | 3.4  | 4.5  | 6.3  | 2.4  | 3.6  | 4.3  | 2.0  | 3.23 | 6.4  | 2.5  | 3.7  | 8.6  | 2.9  | 4.1  | 62.7  |
| 2.3960     | 20   | 4.4  | 5.6  | 17.0 | 4.1  | 5.2  | 28.3 | 5.3  | 6.4  | 21.0 | 4.6  | 5.7  | 25.8 | 5.1  | 6.1  | 31.8 | 5.6  | 6.7  | 32.2 | 5.6  | 6.7  | 196.0 |
| 2.6454     | 5.2  | 2.2  | 3.4  | 5.9  | 2.4  | 3.6  | 12.2 | 3.4  | 4.6  | 0.9  | 0.8  | 2.3  | 1.7  | 1.2  | 2.5  | 10.5 | 3.2  | 4.3  | 4.2  | 2.0  | 3.2  | 45.8  |
| 2.9500     | 0    | 0    | 1.0  | 0    | 0    | 1.0  | 0    | 0    | 1.0  | 3.4  | 1.8  | 3.0  | 1.5  | 1.1  | 2.5  | 3.2  | 1.7  | 3.0  | 0    | 0    | 1.0  | 8.1   |

| $\sqrt{s}$ | BIN1   | BIN2   | BIN3   | BIN4   | BIN5   | BIN6   | BIN7   |
|------------|--------|--------|--------|--------|--------|--------|--------|
| 2.0000     | 0.0238 | 0.0232 | 0.0232 | 0.0230 | 0.0234 | 0.0239 | 0.0246 |
| 2.0500     | 0.0250 | 0.0230 | 0.0227 | 0.0209 | 0.0208 | 0.0232 | 0.0242 |
| 2.1250     | 0.0224 | 0.0214 | 0.0195 | 0.0183 | 0.0200 | 0.021  | 0.0221 |
| 2.1500     | 0.0217 | 0.0194 | 0.0192 | 0.0177 | 0.0183 | 0.0220 | 0.0217 |
| 2.1750     | 0.0206 | 0.0188 | 0.0169 | 0.0167 | 0.0170 | 0.0195 | 0.0205 |
| 2.2000     | 0.0194 | 0.0176 | 0.0163 | 0.0162 | 0.0180 | 0.0187 | 0.0207 |
| 2.2324     | 0.0209 | 0.0188 | 0.0160 | 0.0171 | 0.0180 | 0.0183 | 0.0209 |
| 2.3904     | 0.0226 | 0.0219 | 0.0186 | 0.0179 | 0.0201 | 0.0210 | 0.0232 |
| 2.3864     | 0.0254 | 0.0234 | 0.0223 | 0.0230 | 0.0224 | 0.0248 | 0.0264 |
| 2.3960     | 0.0271 | 0.0242 | 0.0224 | 0.0207 | 0.0224 | 0.0244 | 0.0255 |
| 2.6454     | 0.0124 | 0.0108 | 0.0111 | 0.0096 | 0.0112 | 0.0109 | 0.0123 |
| 2.9500     | 0.0108 | 0.0126 | 0.0101 | 0.0096 | 0.0111 | 0.0122 | 0.0116 |

TABLE XII. DATA:  $\mathcal{E}_{MC}$  @CatA

| $\sqrt{s}$ | BIN1   | BIN2   | BIN3   | BIN4   | BIN5   | BIN6   | BIN7   |
|------------|--------|--------|--------|--------|--------|--------|--------|
| 2.0000     | 0.0066 | 0.0062 | 0.0064 | 0.0061 | 0.0058 | 0.0060 | 0.0069 |
| 2.0500     | 0.0095 | 0.0142 | 0.0136 | 0.0139 | 0.0134 | 0.0141 | 0.0099 |
| 2.1250     | 0.0187 | 0.0269 | 0.0278 | 0.0280 | 0.0277 | 0.0264 | 0.0192 |
| 2.1500     | 0.0226 | 0.0282 | 0.0327 | 0.0306 | 0.0321 | 0.0312 | 0.0233 |
| 2.1750     | 0.0250 | 0.0323 | 0.0342 | 0.0346 | 0.0343 | 0.0323 | 0.0231 |
| 2.2000     | 0.0284 | 0.0364 | 0.0374 | 0.0374 | 0.0371 | 0.0365 | 0.0293 |
| 2.2324     | 0.0283 | 0.0372 | 0.0381 | 0.0396 | 0.0383 | 0.0373 | 0.029  |
| 2.3094     | 0.0349 | 0.0397 | 0.0408 | 0.0412 | 0.0417 | 0.0419 | 0.0324 |
| 2.3864     | 0.0420 | 0.0515 | 0.0511 | 0.0496 | 0.0535 | 0.0513 | 0.0435 |
| 2.3960     | 0.0426 | 0.0489 | 0.0503 | 0.0500 | 0.0523 | 0.0506 | 0.0417 |
| 2.6454     | 0.0427 | 0.0530 | 0.0527 | 0.0518 | 0.0554 | 0.0520 | 0.0425 |
| 2.9500     | 0.0424 | 0.0533 | 0.0577 | 0.0523 | 0.0548 | 0.0557 | 0.0428 |

TABLE XIII. DATA:  $\mathcal{E}_{MC}$  @CatB

| $\sqrt{s}$ | BIN1   | BIN2   | BIN3   | BIN4   | BIN5   | BIN6   | BIN7   |
|------------|--------|--------|--------|--------|--------|--------|--------|
| 2.0000     | 0.0051 | 0.0072 | 0.0077 | 0.0067 | 0.0071 | 0.0079 | 0.0058 |
| 2.0500     | 0.0130 | 0.0161 | 0.0162 | 0.0149 | 0.0166 | 0.0167 | 0.0138 |
| 2.1250     | 0.0233 | 0.0289 | 0.0315 | 0.0274 | 0.0309 | 0.0299 | 0.0246 |
| 2.1500     | 0.0258 | 0.0326 | 0.0337 | 0.0323 | 0.0343 | 0.0359 | 0.0295 |
| 2.1750     | 0.0293 | 0.0366 | 0.0371 | 0.0322 | 0.0377 | 0.0331 | 0.0285 |
| 2.2000     | 0.0301 | 0.0383 | 0.0364 | 0.0406 | 0.0396 | 0.0406 | 0.0332 |
| 2.2324     | 0.0356 | 0.0419 | 0.0434 | 0.0384 | 0.0446 | 0.0428 | 0.0359 |
| 2.3094     | 0.0381 | 0.0429 | 0.0441 | 0.0405 | 0.0434 | 0.0430 | 0.0372 |
| 2.3864     | 0.0464 | 0.0523 | 0.0510 | 0.0496 | 0.0529 | 0.0564 | 0.0480 |
| 2.3960     | 0.0432 | 0.0527 | 0.0508 | 0.0498 | 0.0515 | 0.0536 | 0.0475 |
| 2.6454     | 0.0567 | 0.0671 | 0.0659 | 0.0592 | 0.0639 | 0.0661 | 0.0568 |
| 2.9500     | 0.0489 | 0.0604 | 0.0605 | 0.0561 | 0.0600 | 0.0633 | 0.0511 |

TABLE XIV. DATA:  $\mathcal{E}_{MC}$  @CatC

| $\sqrt{s}$ | BIN1 | Err1 | BIN2 | Err2 | BIN3 | Err3 | BIN4 | Err4 | BIN5 | Err5 | BIN6 | Err6 | BIN7 | Err7 |
|------------|------|------|------|------|------|------|------|------|------|------|------|------|------|------|
| 2.0000     | 1.23 | 0.10 | 1.04 | 0.09 | 1.29 | 0.12 | 0.95 | 0.08 | 1.20 | 0.10 | 1.11 | 0.09 | 1.13 | 0.09 |
| 2.0500     | 1.00 | 0.07 | 1.10 | 0.07 | 1.17 | 0.09 | 0.97 | 0.07 | 0.97 | 0.07 | 1.11 | 0.08 | 1.27 | 0.08 |
| 2.1250     | 1.01 | 0.06 | 0.99 | 0.06 | 0.95 | 0.06 | 1.00 | 0.06 | 0.97 | 0.06 | 1.02 | 0.06 | 1.03 | 0.06 |
| 2.1500     | 0.95 | 0.05 | 1.05 | 0.06 | 0.92 | 0.05 | 0.88 | 0.05 | 0.92 | 0.06 | 0.99 | 0.06 | 1.02 | 0.06 |
| 2.1750     | 0.94 | 0.05 | 0.99 | 0.06 | 1.03 | 0.06 | 0.97 | 0.06 | 0.90 | 0.05 | 1.02 | 0.06 | 0.94 | 0.05 |
| 2.2000     | 0.98 | 0.05 | 0.93 | 0.05 | 0.93 | 0.05 | 0.98 | 0.06 | 1.08 | 0.06 | 0.97 | 0.05 | 0.94 | 0.05 |
| 2.2324     | 1.01 | 0.05 | 1.03 | 0.06 | 0.99 | 0.05 | 0.93 | 0.05 | 1.00 | 0.06 | 0.95 | 0.05 | 1.09 | 0.06 |
| 2.3904     | 0.92 | 0.05 | 0.98 | 0.05 | 0.96 | 0.05 | 0.95 | 0.05 | 0.99 | 0.05 | 0.98 | 0.05 | 1.04 | 0.05 |
| 2.3864     | 0.98 | 0.05 | 0.91 | 0.04 | 1.03 | 0.05 | 0.97 | 0.05 | 0.87 | 0.04 | 0.94 | 0.05 | 0.98 | 0.05 |
| 2.3960     | 0.94 | 0.04 | 0.89 | 0.04 | 1.01 | 0.05 | 0.94 | 0.04 | 0.90 | 0.04 | 0.95 | 0.04 | 0.96 | 0.04 |
| 2.6454     | 0.91 | 0.04 | 0.80 | 0.03 | 0.89 | 0.03 | 0.74 | 0.03 | 0.85 | 0.03 | 0.84 | 0.03 | 0.85 | 0.04 |
| 2.9500     | 0.80 | 0.03 | 0.81 | 0.03 | 0.75 | 0.03 | 0.73 | 0.03 | 0.77 | 0.03 | 0.78 | 0.03 | 0.86 | 0.04 |

TABLE XV. DATA:  $\mathcal{C}_{dm}$  @CatA

| $\sqrt{s}$ | BIN1 | Err1 | BIN2 | Err2 | BIN3 | Err3 | BIN4 | Err4 | BIN5 | Err5 | BIN6 | Err6 | BIN7 | Err7 |
|------------|------|------|------|------|------|------|------|------|------|------|------|------|------|------|
| 2.0000     | 0.92 | 0.01 | 0.82 | 0.01 | 0.79 | 0.01 | 0.74 | 0.01 | 0.72 | 0.01 | 0.73 | 0.01 | 0.76 | 0.01 |
| 2.0500     | 0.67 | 0.01 | 0.69 | 0.01 | 0.68 | 0.01 | 0.67 | 0.01 | 0.67 | 0.01 | 0.68 | 0.01 | 0.69 | 0.01 |
| 2.1250     | 0.79 | 0.01 | 0.78 | 0.01 | 0.76 | 0.01 | 0.76 | 0.01 | 0.75 | 0.01 | 0.77 | 0.01 | 0.78 | 0.01 |
| 2.1500     | 0.84 | 0.04 | 0.82 | 0.05 | 0.80 | 0.05 | 0.79 | 0.05 | 0.78 | 0.05 | 0.79 | 0.05 | 0.80 | 0.04 |
| 2.1750     | 0.86 | 0.04 | 0.83 | 0.05 | 0.81 | 0.05 | 0.80 | 0.05 | 0.80 | 0.05 | 0.80 | 0.05 | 0.81 | 0.04 |
| 2.2000     | 0.83 | 0.04 | 0.81 | 0.05 | 0.81 | 0.05 | 0.80 | 0.05 | 0.80 | 0.04 | 0.81 | 0.05 | 0.81 | 0.04 |
| 2.2324     | 0.86 | 0.04 | 0.84 | 0.05 | 0.83 | 0.05 | 0.82 | 0.05 | 0.82 | 0.05 | 0.82 | 0.05 | 0.83 | 0.04 |
| 2.3094     | 0.88 | 0.04 | 0.86 | 0.04 | 0.85 | 0.04 | 0.85 | 0.04 | 0.84 | 0.04 | 0.84 | 0.04 | 0.86 | 0.04 |
| 2.3864     | 0.88 | 0.01 | 0.89 | 0.01 | 0.88 | 0.01 | 0.88 | 0.01 | 0.88 | 0.01 | 0.88 | 0.01 | 0.89 | 0.01 |
| 2.3960     | 0.88 | 0.01 | 0.89 | 0.01 | 0.88 | 0.01 | 0.88 | 0.01 | 0.88 | 0.01 | 0.88 | 0.01 | 0.89 | 0.01 |
| 2.6454     | 0.86 | 0.01 | 0.84 | 0.01 | 0.84 | 0.01 | 0.83 | 0.01 | 0.83 | 0.01 | 0.83 | 0.01 | 0.84 | 0.01 |
| 2.9500     | 0.80 | 0.01 | 0.79 | 0.01 | 0.80 | 0.01 | 0.80 | 0.01 | 0.80 | 0.01 | 0.80 | 0.01 | 0.81 | 0.01 |

TABLE XVI. DATA:  $\mathcal{C}_{dm}$  @CatB

| $\sqrt{s}$ | BIN1 | Err1 | BIN2 | Err2 | BIN3 | Err3 | BIN4 | Err4 | BIN5 | Err5 | BIN6 | Err6 | BIN7 | Err7 |
|------------|------|------|------|------|------|------|------|------|------|------|------|------|------|------|
| 2.0000     | 1.23 | 0.13 | 1.33 | 0.12 | 1.38 | 0.14 | 1.22 | 0.12 | 1.29 | 0.13 | 1.32 | 0.12 | 1.78 | 0.18 |
| 2.0500     | 1.21 | 0.07 | 1.29 | 0.07 | 1.27 | 0.07 | 1.19 | 0.07 | 1.28 | 0.07 | 1.22 | 0.07 | 1.34 | 0.08 |
| 2.1250     | 1.24 | 0.06 | 1.28 | 0.06 | 1.22 | 0.06 | 1.17 | 0.06 | 1.24 | 0.06 | 1.20 | 0.06 | 1.31 | 0.07 |
| 2.1500     | 1.30 | 0.07 | 1.24 | 0.06 | 1.18 | 0.06 | 1.16 | 0.06 | 1.16 | 0.06 | 1.19 | 0.06 | 1.35 | 0.07 |
| 2.1750     | 1.31 | 0.08 | 1.24 | 0.06 | 1.17 | 0.06 | 1.16 | 0.06 | 1.15 | 0.06 | 1.19 | 0.06 | 1.35 | 0.08 |
| 2.2000     | 1.31 | 0.08 | 1.23 | 0.06 | 1.17 | 0.06 | 1.16 | 0.06 | 1.15 | 0.06 | 1.19 | 0.06 | 1.35 | 0.08 |
| 2.2324     | 1.29 | 0.05 | 1.20 | 0.04 | 1.17 | 0.04 | 1.13 | 0.04 | 1.13 | 0.04 | 1.21 | 0.04 | 1.33 | 0.05 |
| 2.3094     | 1.27 | 0.07 | 1.21 | 0.06 | 1.18 | 0.06 | 1.11 | 0.06 | 1.13 | 0.06 | 1.28 | 0.06 | 1.34 | 0.07 |
| 2.3864     | 1.14 | 0.06 | 1.15 | 0.05 | 1.13 | 0.05 | 1.13 | 0.05 | 1.11 | 0.05 | 1.18 | 0.05 | 1.24 | 0.06 |
| 2.3960     | 1.15 | 0.05 | 1.15 | 0.05 | 1.13 | 0.05 | 1.13 | 0.05 | 1.12 | 0.05 | 1.18 | 0.05 | 1.24 | 0.06 |
| 2.6454     | 0.95 | 0.03 | 1.03 | 0.03 | 1.07 | 0.03 | 1.03 | 0.03 | 1.0  | 0.03 | 0.96 | 0.03 | 1.01 | 0.03 |
| 2.9500     | 1.09 | 0.06 | 1.06 | 0.05 | 1.08 | 0.05 | 1.01 | 0.05 | 1.0  | 0.05 | 1.05 | 0.05 | 1.09 | 0.06 |

TABLE XVII. DATA:  $\mathcal{C}_{dm}$  @CatC

| $\sqrt{s}$ | BIN1  | Err1  | BIN2  | Err2  | BIN3  | Err3  | BIN4  | Err4  | BIN5  | Err5  | BIN6  | Err6  | BIN7  | Err7  |
|------------|-------|-------|-------|-------|-------|-------|-------|-------|-------|-------|-------|-------|-------|-------|
| 2.0000     | 0.983 | 0.007 | 0.981 | 0.007 | 0.982 | 0.007 | 0.978 | 0.007 | 0.982 | 0.007 | 0.985 | 0.007 | 0.984 | 0.007 |
| 2.0500     | 1.079 | 0.008 | 1.074 | 0.008 | 1.072 | 0.008 | 1.079 | 0.008 | 1.075 | 0.008 | 1.081 | 0.008 | 1.079 | 0.008 |
| 2.1250     | 1.244 | 0.009 | 1.227 | 0.009 | 1.222 | 0.009 | 1.218 | 0.009 | 1.220 | 0.009 | 1.221 | 0.009 | 1.243 | 0.009 |
| 2.1500     | 1.279 | 0.010 | 1.270 | 0.010 | 1.261 | 0.010 | 1.249 | 0.010 | 1.255 | 0.010 | 1.267 | 0.010 | 1.288 | 0.010 |
| 2.1750     | 1.310 | 0.010 | 1.291 | 0.010 | 1.279 | 0.010 | 1.268 | 0.010 | 1.273 | 0.010 | 1.287 | 0.010 | 1.315 | 0.010 |
| 2.2000     | 1.316 | 0.010 | 1.286 | 0.010 | 1.278 | 0.010 | 1.266 | 0.010 | 1.271 | 0.010 | 1.287 | 0.010 | 1.319 | 0.010 |
| 2.2324     | 1.287 | 0.010 | 1.248 | 0.010 | 1.247 | 0.010 | 1.223 | 0.010 | 1.231 | 0.010 | 1.256 | 0.010 | 1.281 | 0.010 |
| 2.3094     | 1.147 | 0.009 | 1.124 | 0.009 | 1.106 | 0.009 | 1.097 | 0.008 | 1.115 | 0.009 | 1.123 | 0.009 | 1.155 | 0.009 |
| 2.3864     | 1.112 | 0.008 | 1.082 | 0.008 | 1.070 | 0.008 | 1.063 | 0.008 | 1.071 | 0.008 | 1.085 | 0.008 | 1.109 | 0.008 |
| 2.3960     | 1.118 | 0.009 | 1.093 | 0.009 | 1.079 | 0.009 | 1.078 | 0.009 | 1.082 | 0.009 | 1.095 | 0.009 | 1.122 | 0.009 |
| 2.6454     | 1.532 | 0.013 | 1.439 | 0.013 | 1.380 | 0.012 | 1.374 | 0.012 | 1.369 | 0.012 | 1.434 | 0.012 | 1.526 | 0.013 |
| 2.9500     | 2.114 | 0.021 | 1.845 | 0.019 | 1.784 | 0.018 | 1.698 | 0.018 | 1.701 | 0.018 | 1.842 | 0.019 | 2.132 | 0.022 |

TABLE XVIII. DATA:  $(1 + \delta)$  @all categories

| $\sqrt{s}$ | $\mathcal{C}_{trg}^A$ | $\delta\mathcal{C}_{trg}^A$ | $\mathcal{C}_{trg}^B$ | $\delta\mathcal{C}_{trg}^B$ | $\mathcal{C}_{trg}^C$ | $\delta\mathcal{C}_{trg}^C$ | $\mathcal{C}_{ex}^C$ | $\delta\mathcal{C}_{ex}^C$ |
|------------|-----------------------|-----------------------------|-----------------------|-----------------------------|-----------------------|-----------------------------|----------------------|----------------------------|
| 2.0000     | 0.78                  | 0.01                        | 0.87                  | 0.03                        | 0.89                  | 0.03                        | 0.75                 | 0.02                       |
| 2.0500     | 0.78                  | 0.01                        | 0.87                  | 0.02                        | 0.91                  | 0.02                        | 0.75                 | 0.02                       |
| 2.1250     | 0.80                  | 0.01                        | 0.89                  | 0.01                        | 0.93                  | 0.01                        | 0.80                 | 0.01                       |
| 2.1500     | 0.81                  | 0.01                        | 0.90                  | 0.01                        | 0.93                  | 0.01                        | 0.83                 | 0.01                       |
| 2.1750     | 0.79                  | 0.01                        | 0.84                  | 0.01                        | 0.92                  | 0.01                        | 0.86                 | 0.02                       |
| 2.2000     | 0.80                  | 0.01                        | 0.85                  | 0.01                        | 0.92                  | 0.01                        | 0.88                 | 0.02                       |
| 2.2324     | 0.81                  | 0.01                        | 0.85                  | 0.01                        | 0.93                  | 0.01                        | 0.89                 | 0.02                       |
| 2.3094     | 0.83                  | 0.01                        | 0.88                  | 0.01                        | 0.95                  | 0.01                        | 0.90                 | 0.02                       |
| 2.3864     | 0.85                  | 0.01                        | 0.95                  | 0.01                        | 0.96                  | 0.01                        | 0.90                 | 0.02                       |
| 2.3960     | 0.85                  | 0.01                        | 0.94                  | 0.01                        | 0.96                  | 0.01                        | 0.90                 | 0.02                       |
| 2.6454     | 0.93                  | 0.02                        | 0.96                  | 0.01                        | 0.97                  | 0.01                        | 0.90                 | 0.03                       |
| 2.9500     | 0.95                  | 0.02                        | 0.98                  | 0.01                        | 0.98                  | 0.01                        | 0.90                 | 0.05                       |

TABLE XIX. DATA:  $\mathcal{C}_{trg}$  @all categories AND  $\mathcal{C}_{ex}$  @CatC
